# Supplementary material for: PSENet: Progressive Self-Enhancement Network for Unsupervised Extreme-Light Image Enhancement
Source: arXiv:2210.00712 source file (2022-10-03)
Supplement: Supplementary file 1 [file supplementary.pdf]

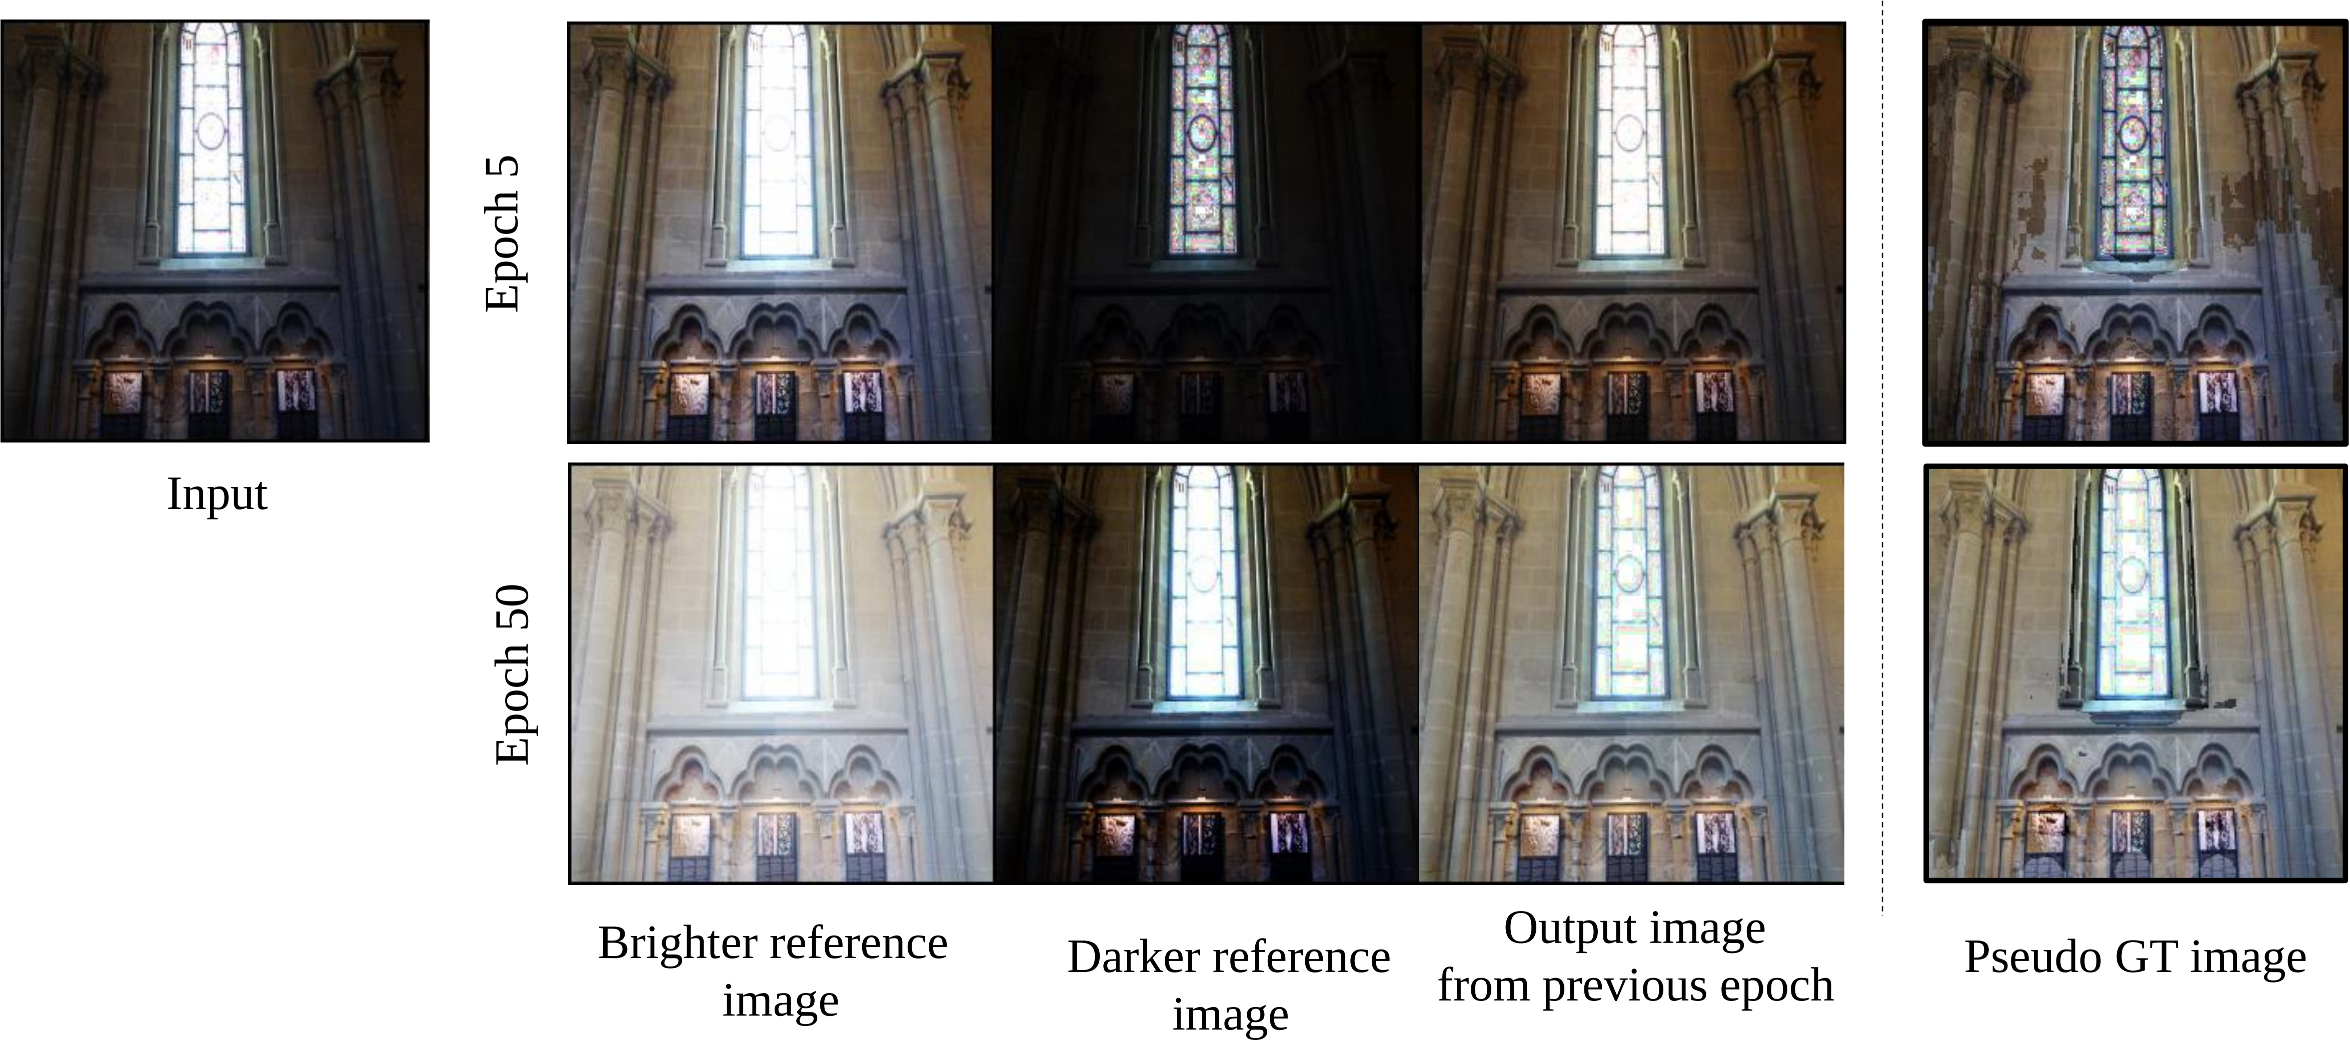
Input
Epoch 5
Epoch 50
Brighter reference image
Darker reference image
Output image from previous epoch
Pseudo GT image

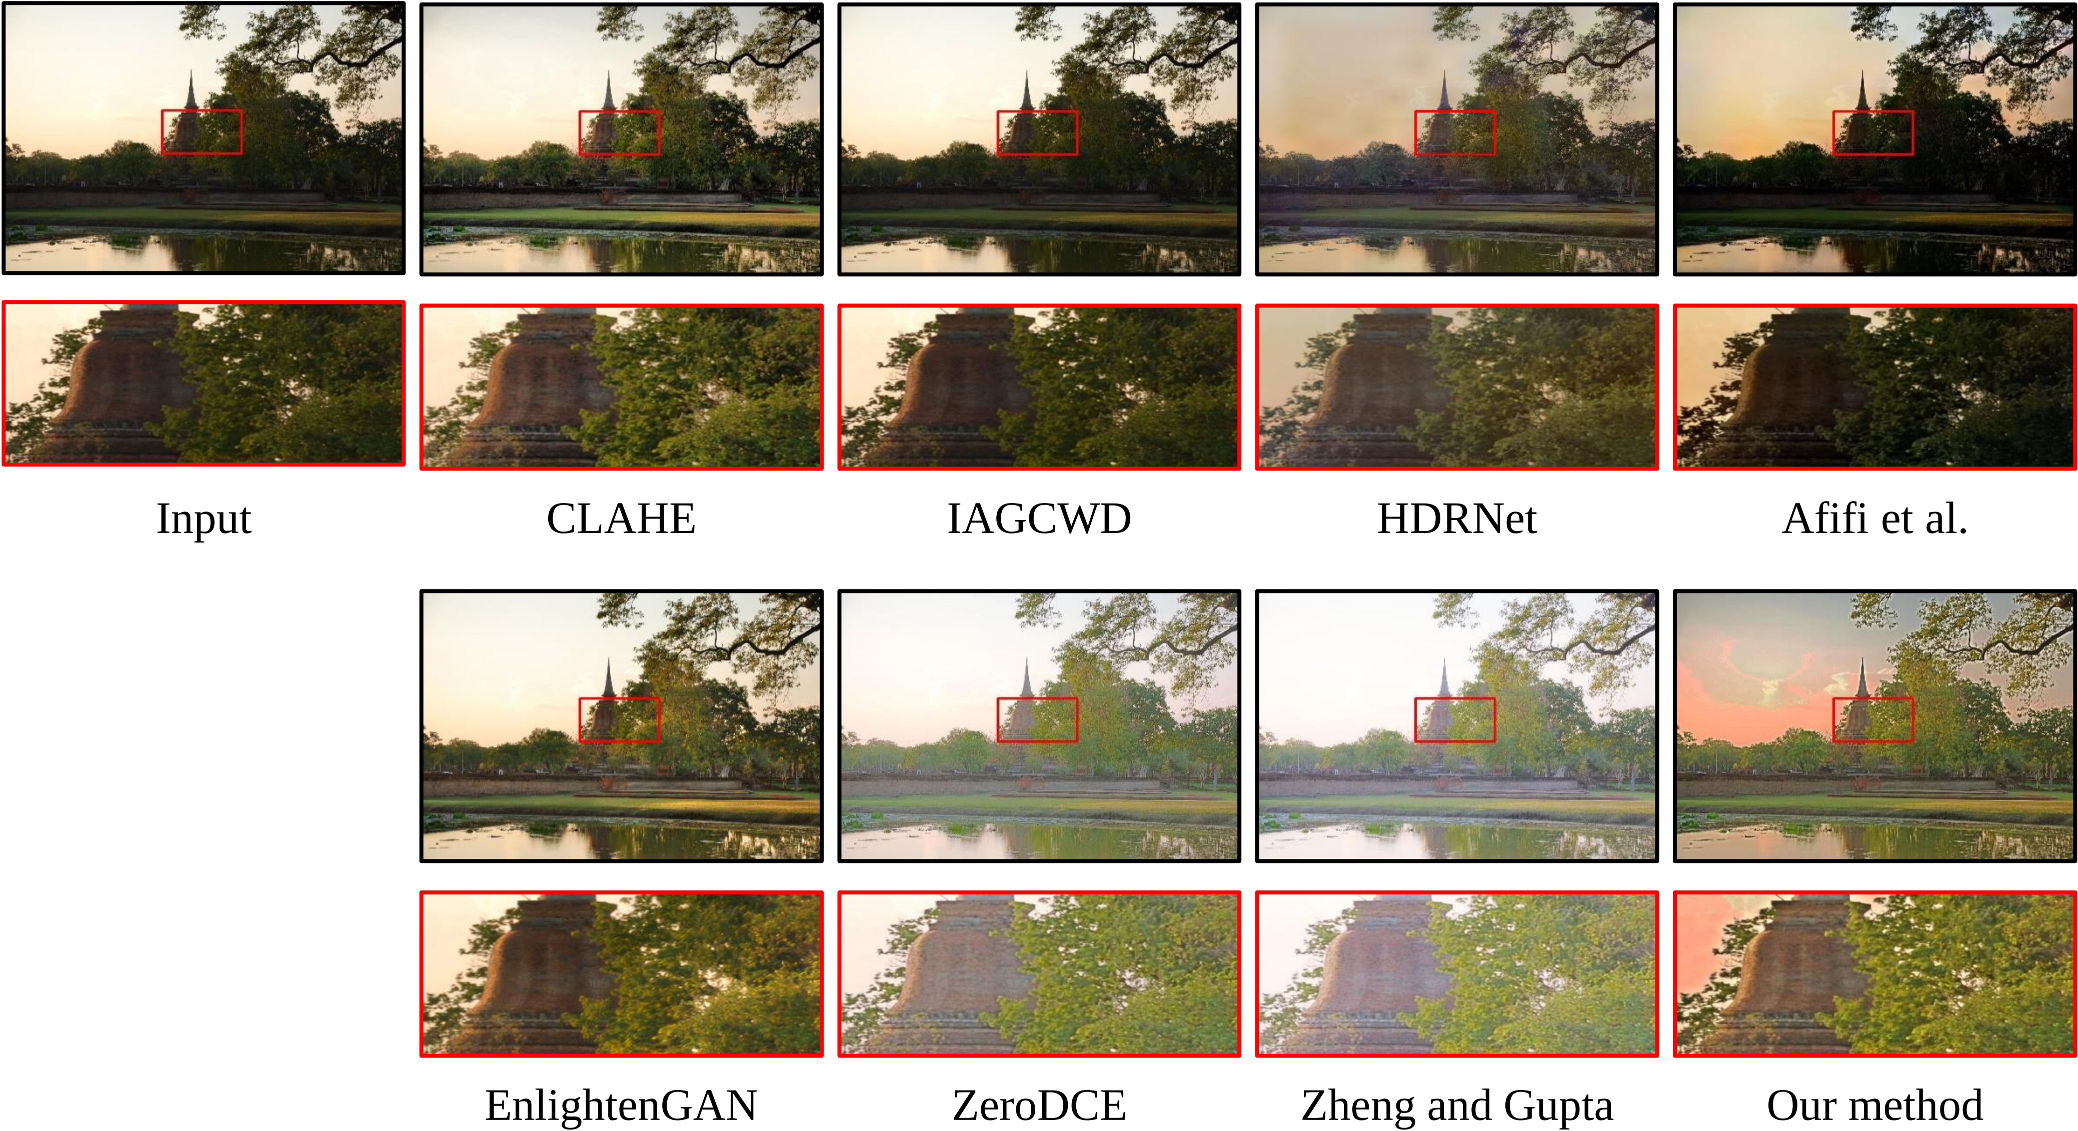
Input
CLAHE
IAGCWD
HDRNet
Afifi et al.
EnlightenGAN
ZeroDCE
Zheng and Gupta
Our method

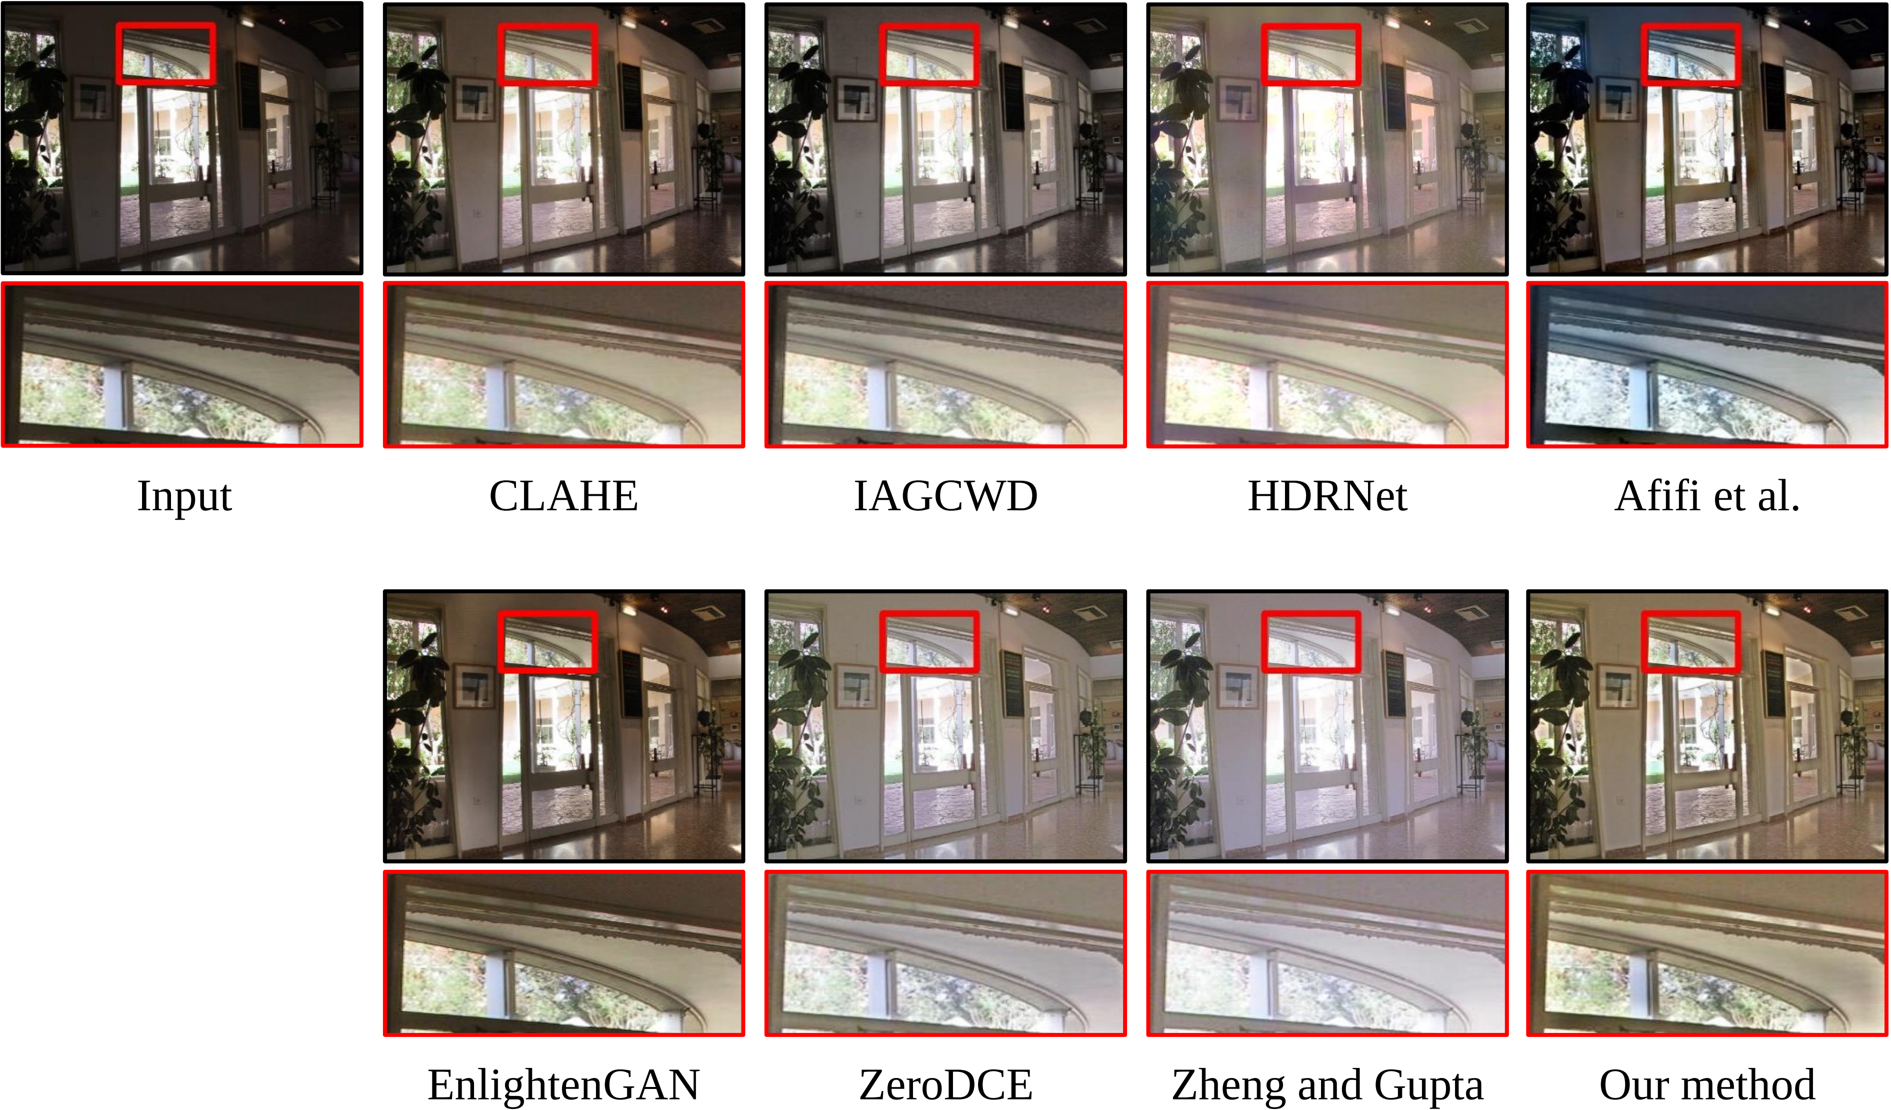
Input
CLAHE
IAGCWD
HDRNet
Afifi et al.
EnlightenGAN
ZeroDCE
Zheng and Gupta
Our method

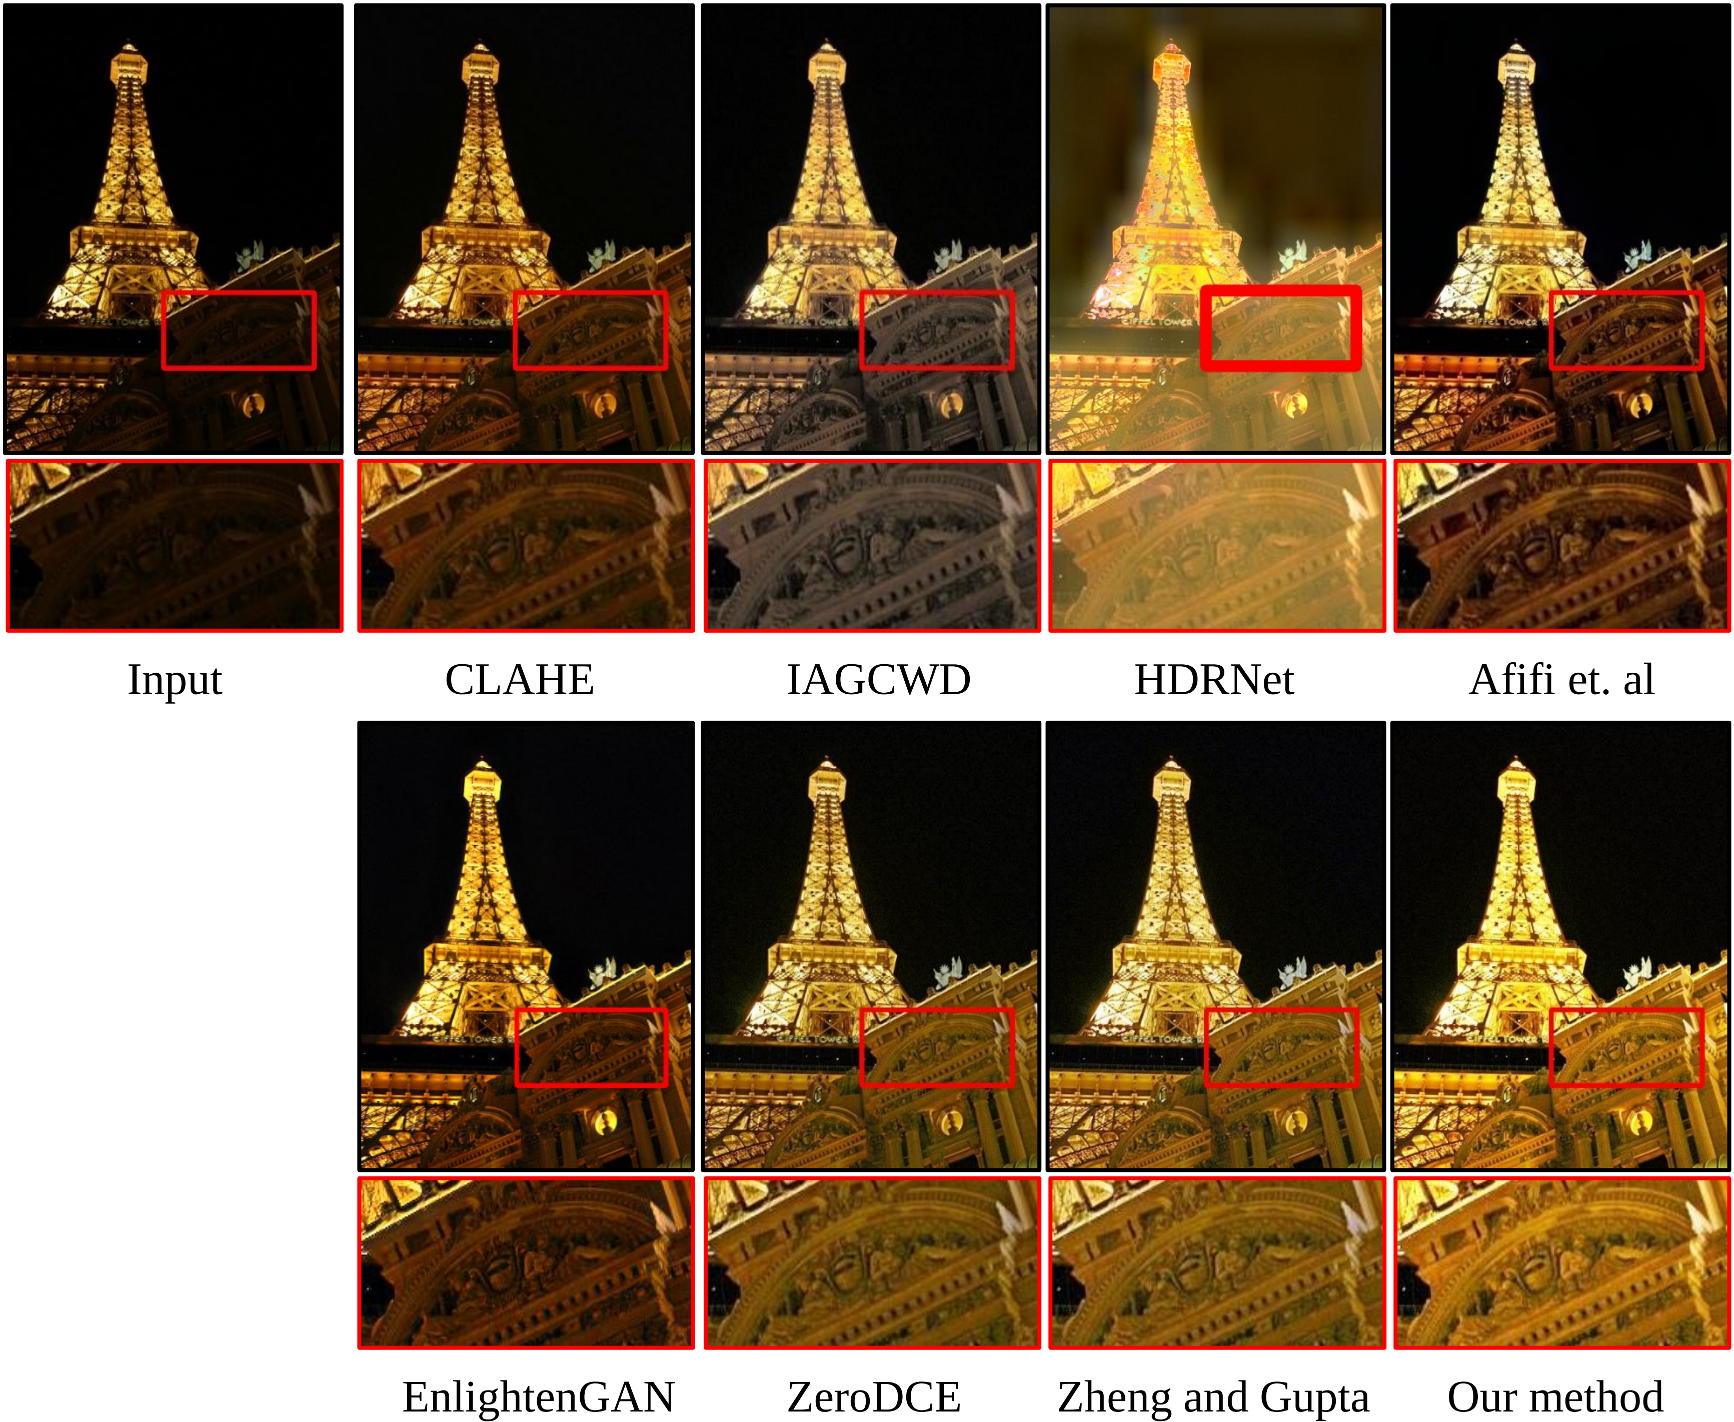
Input
CLAHE
IAGCWD
HDRNet
Afifi et. al
EnlightenGAN
ZeroDCE
Zheng and Gupta
Our method

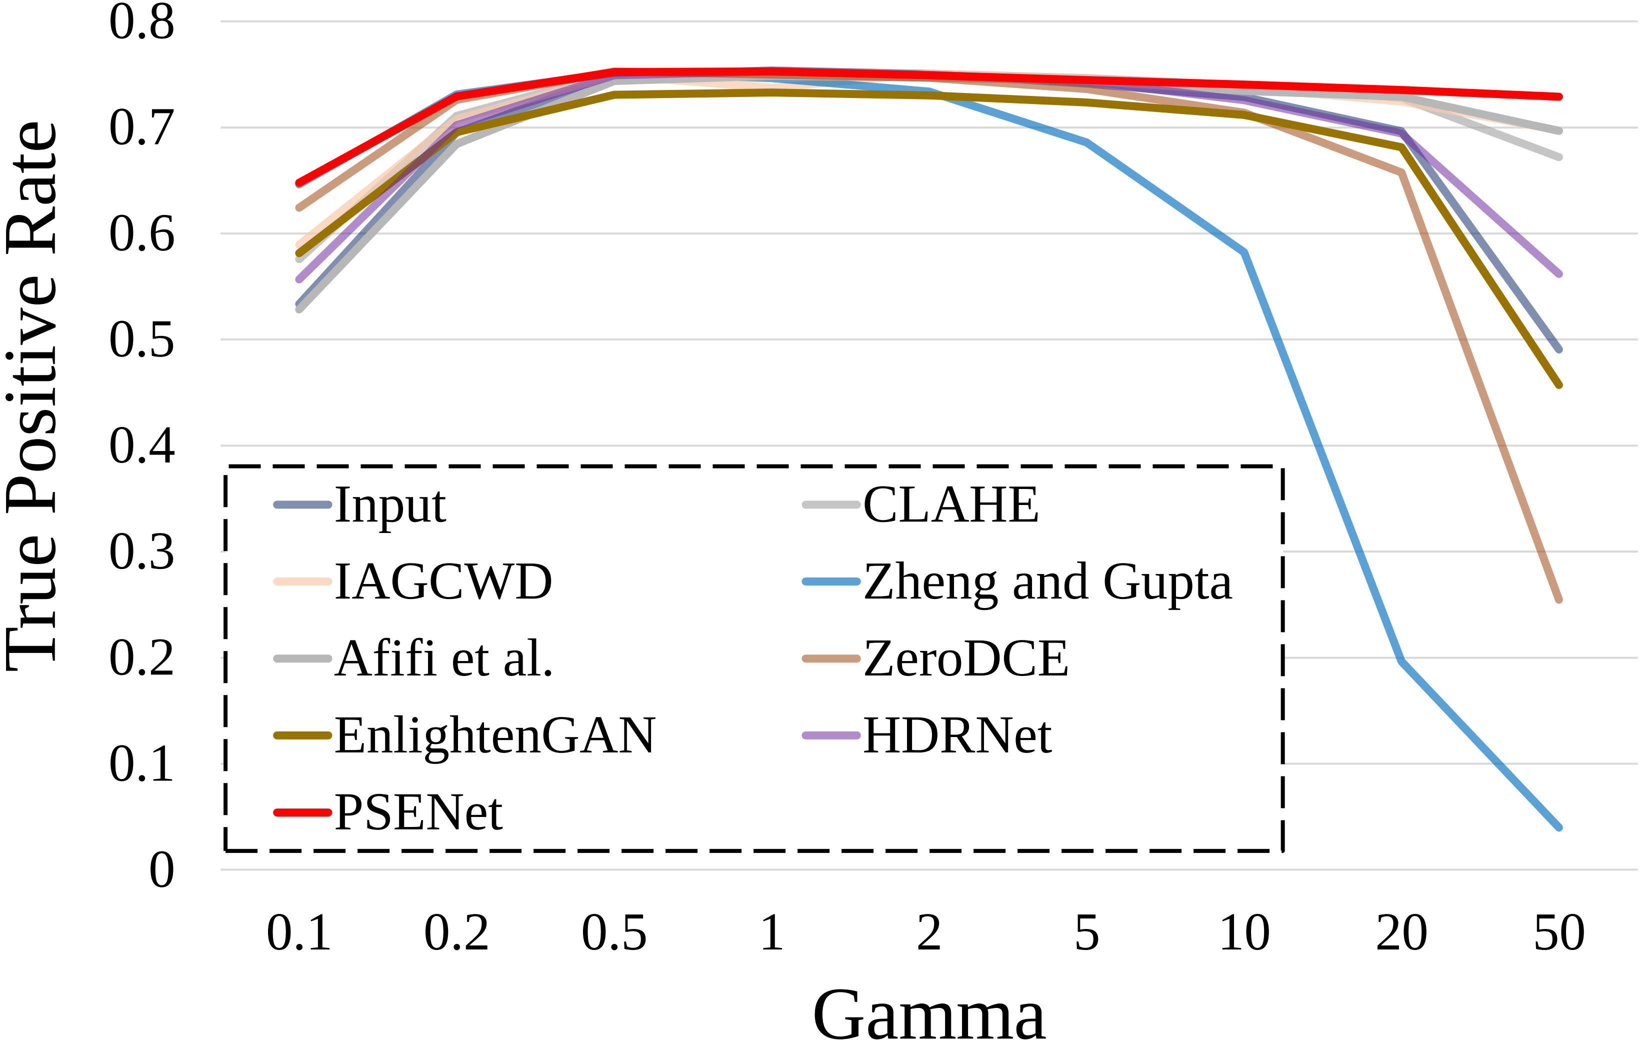

True Positive Rate
0.8
0.7
0.6
0.5
0.4
0.3
0.2
0.1
0
0.1
0.2
0.5
1
2
5
10
20
50
Gamma
Input
CLAHE
IAGCWD
Zheng and Gupta
Afifi et al.
ZeroDCE
EnlightenGAN
HDRNet
PSENet

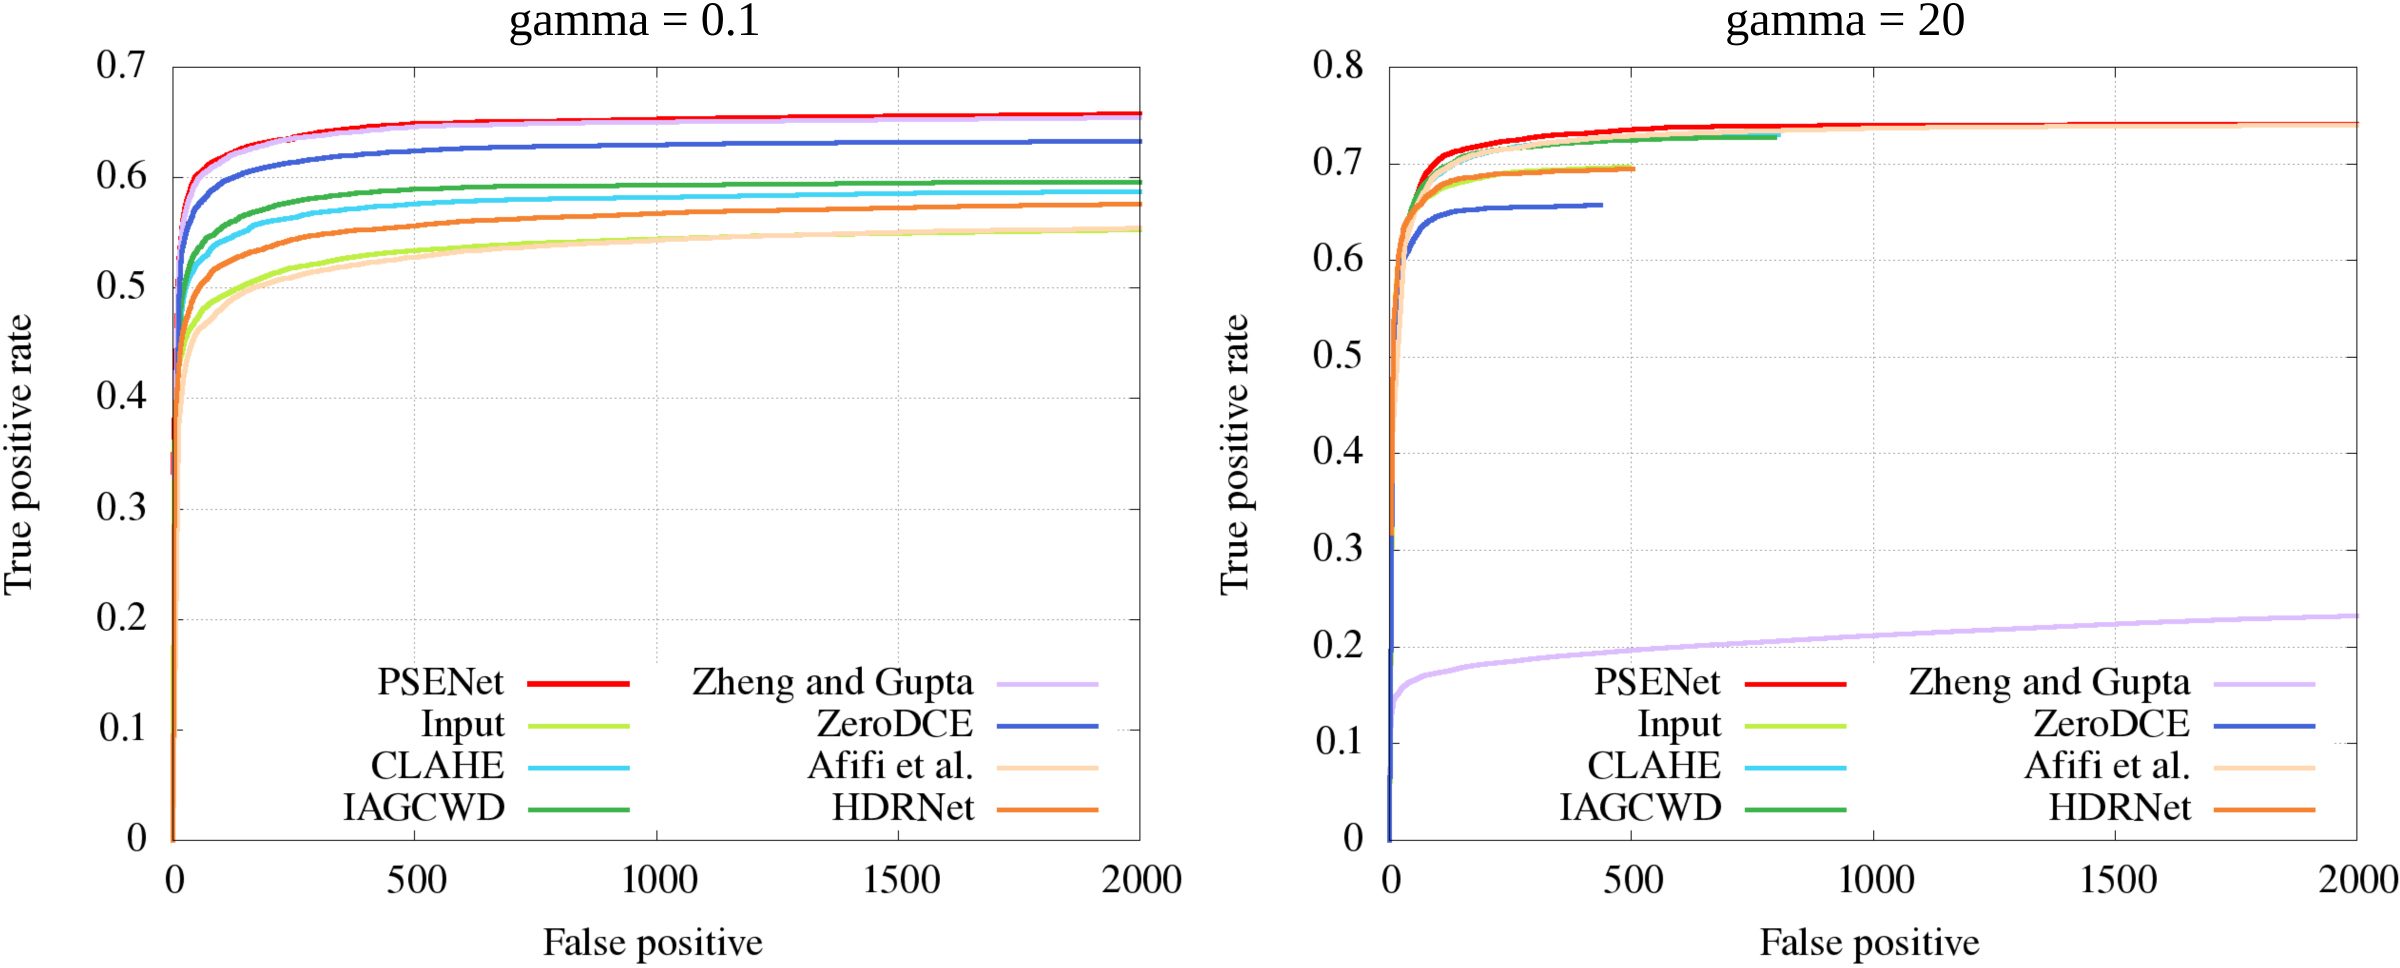
gamma = 0.1
gamma = 20
True positive rate
False positive
0.7
0.6
0.5
0.4
0.3
0.2
0.1
0
0.8
0
500
1000
1500
2000
PSENet
Input
CLAHE
IAGCWD
Zheng and Gupta
ZeroDCE
Afifi et al.
HDRNet

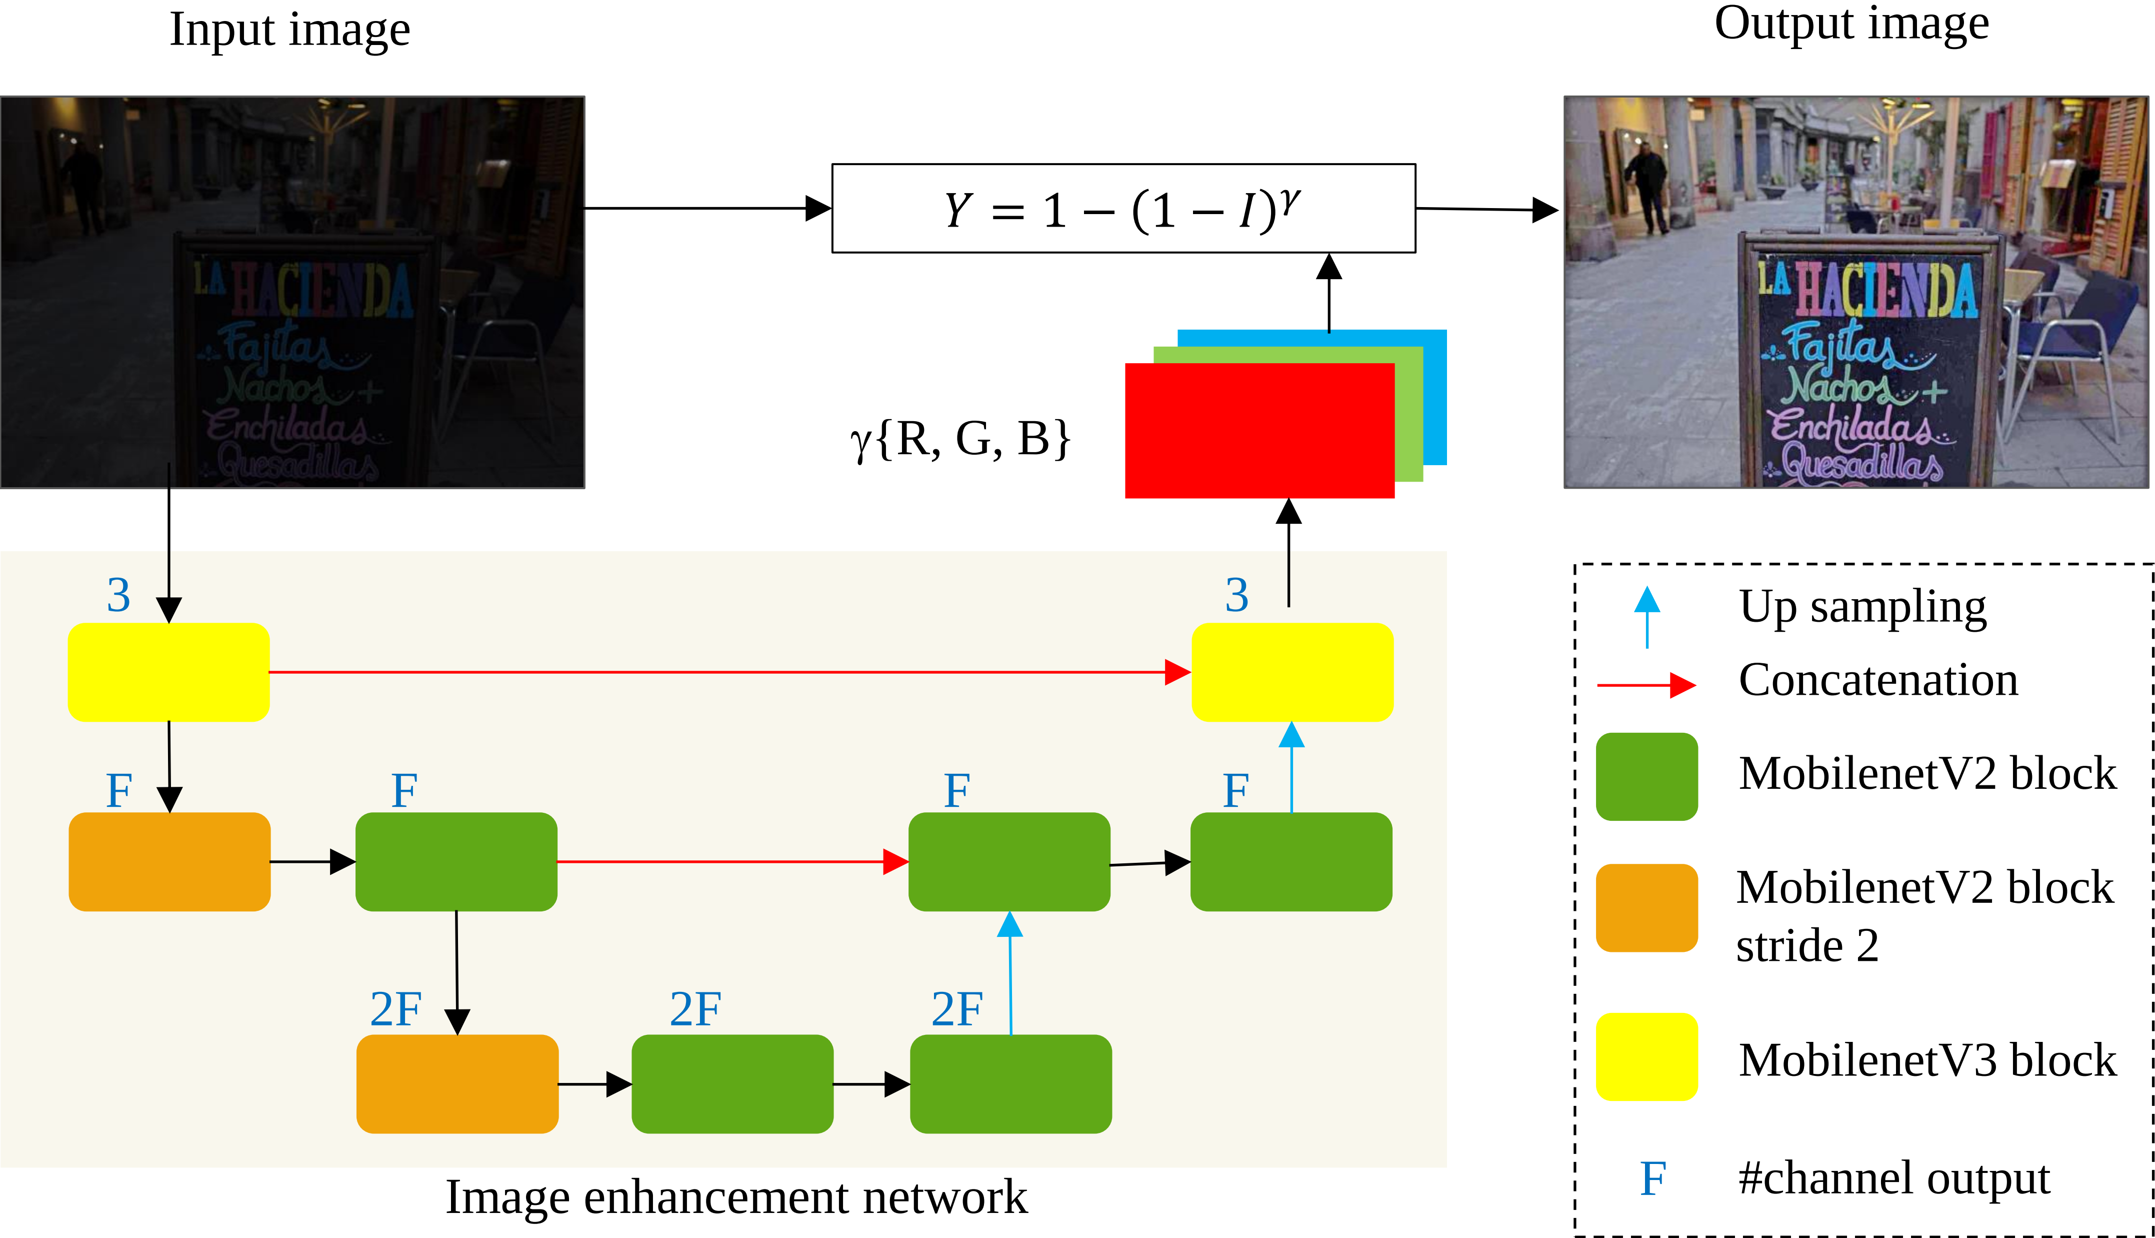

Input image
Output image
$Y = 1 - (1 - I)^{\gamma}$
γ{R, G, B}
LA HACIENDA
Fajitas
Nachos
Enchiladas
Quesadillas
3
F
F
F
F
2F
2F
2F
3
Image enhancement network
Up sampling
Concatenation
MobilenetV2 block
MobilenetV2 block stride 2
MobilenetV3 block
F
#channel output

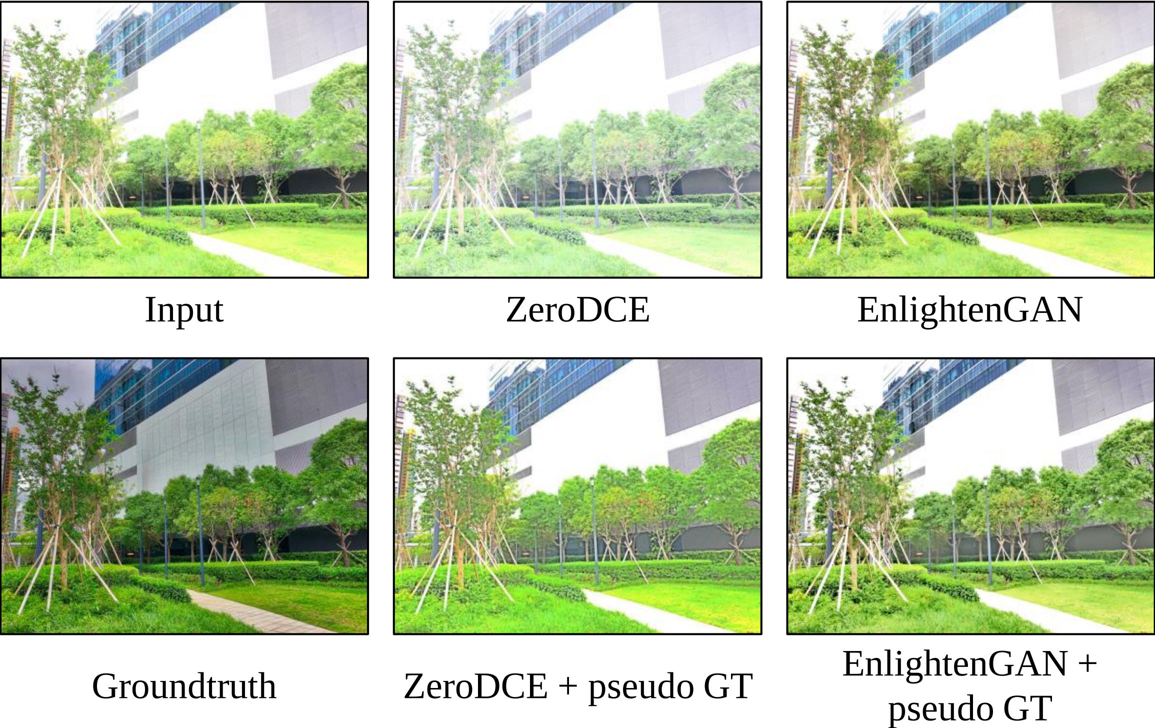
Input
ZeroDCE
EnlightenGAN
Groundtruth
ZeroDCE + pseudo GT
EnlightenGAN + pseudo GT

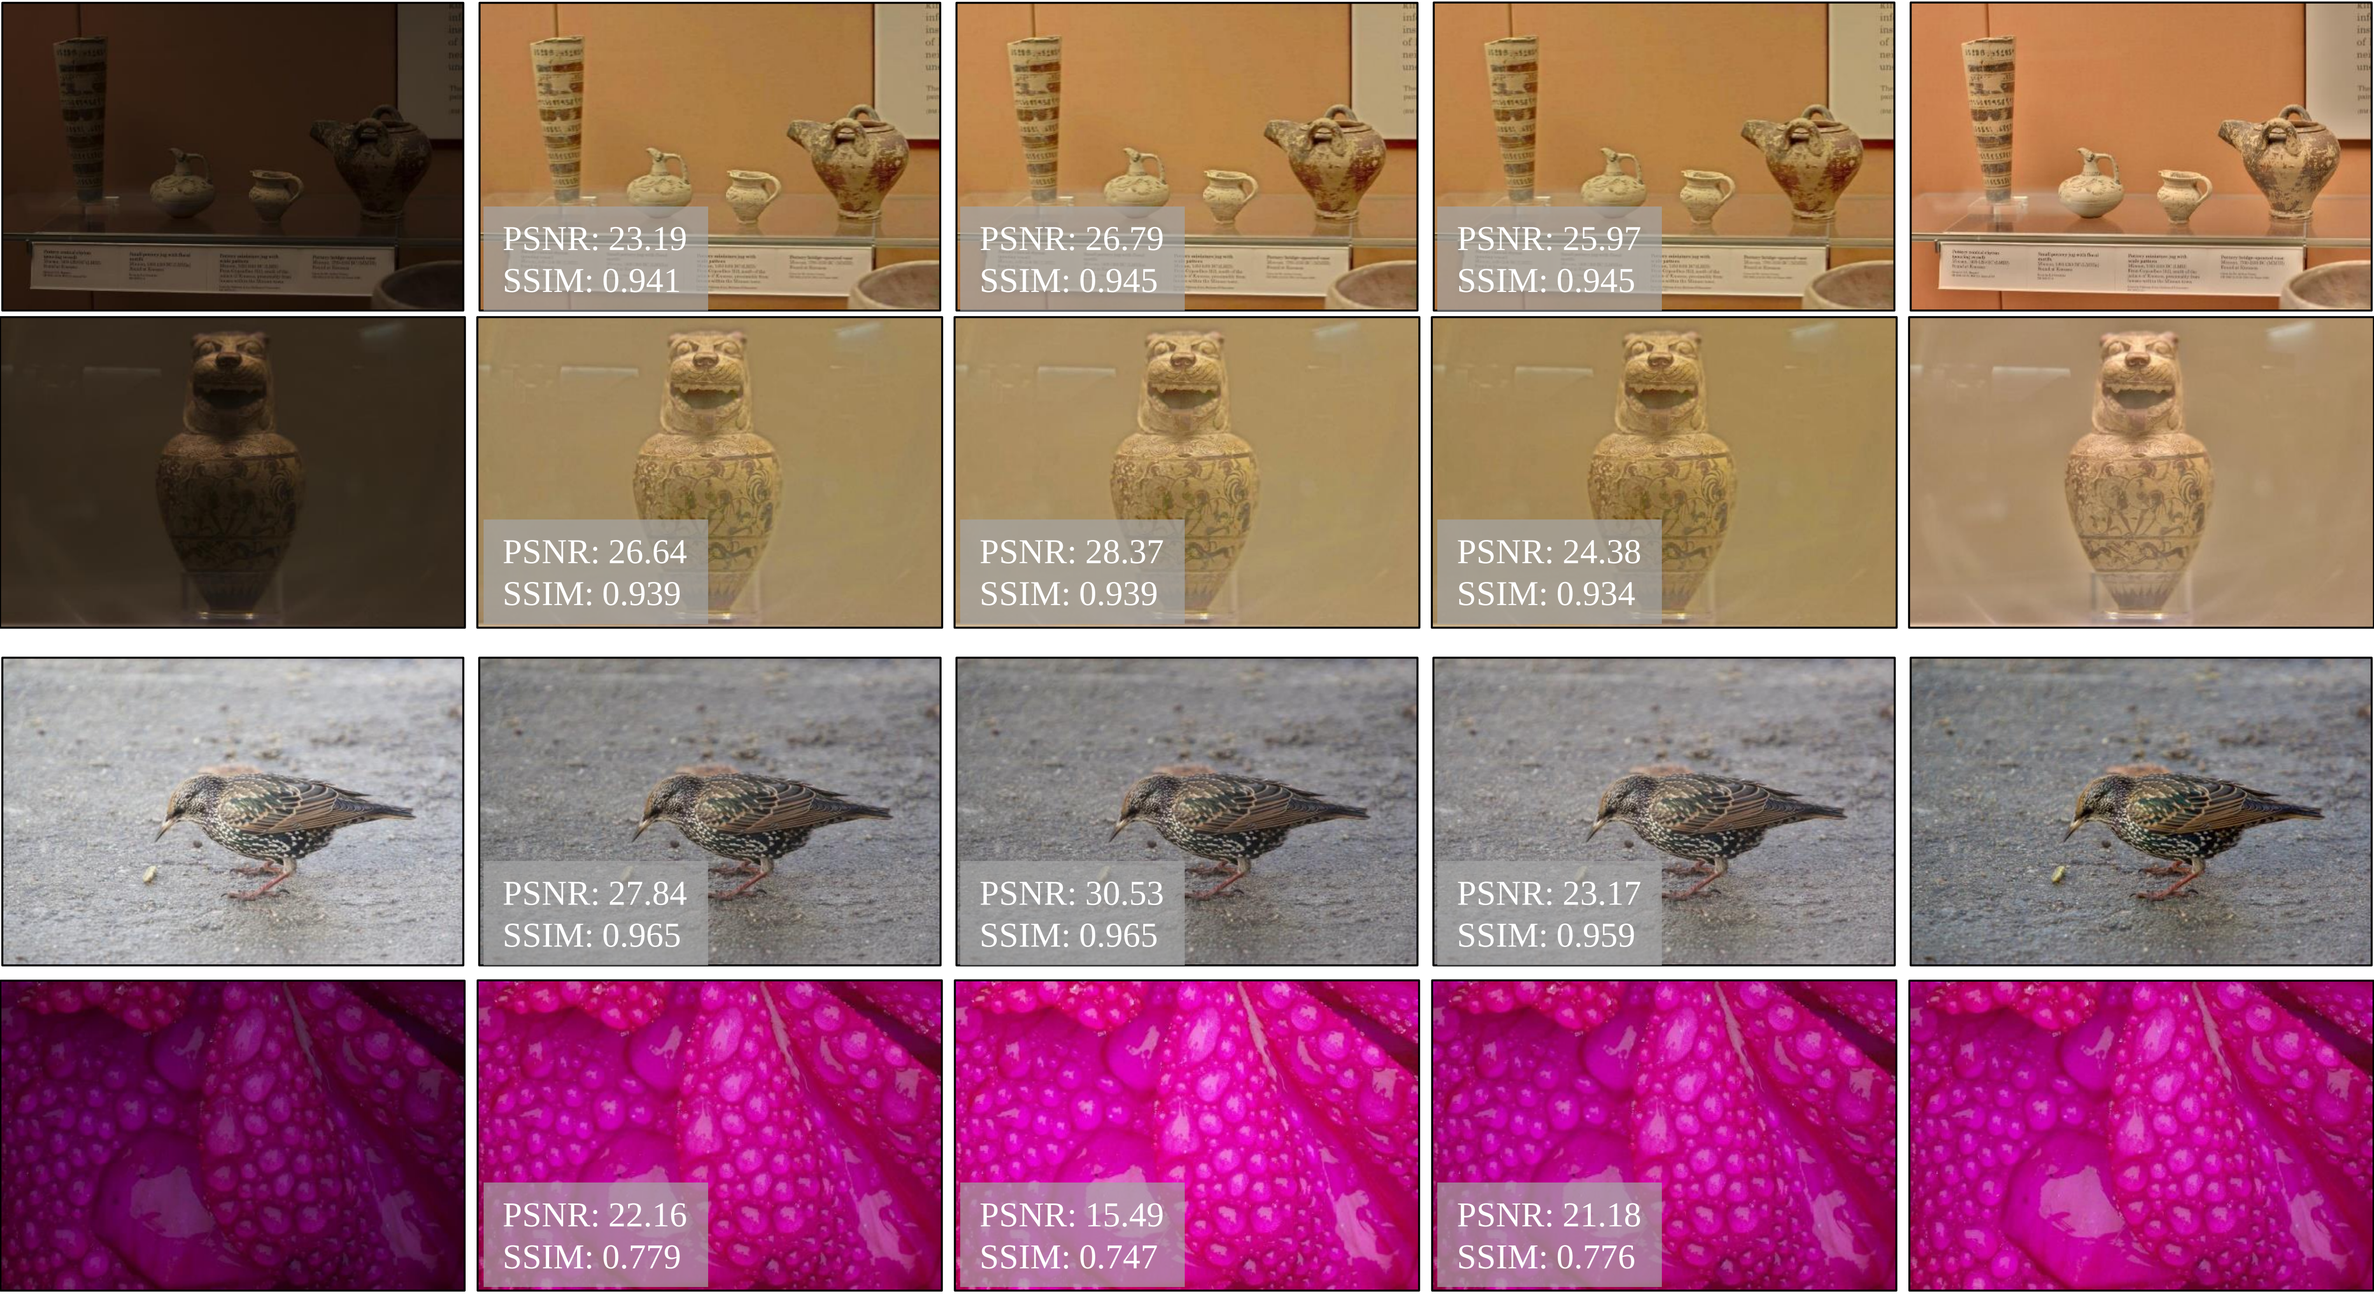


Input # channels x 0.5 # channels x 1 # channels x 2 Ground truth

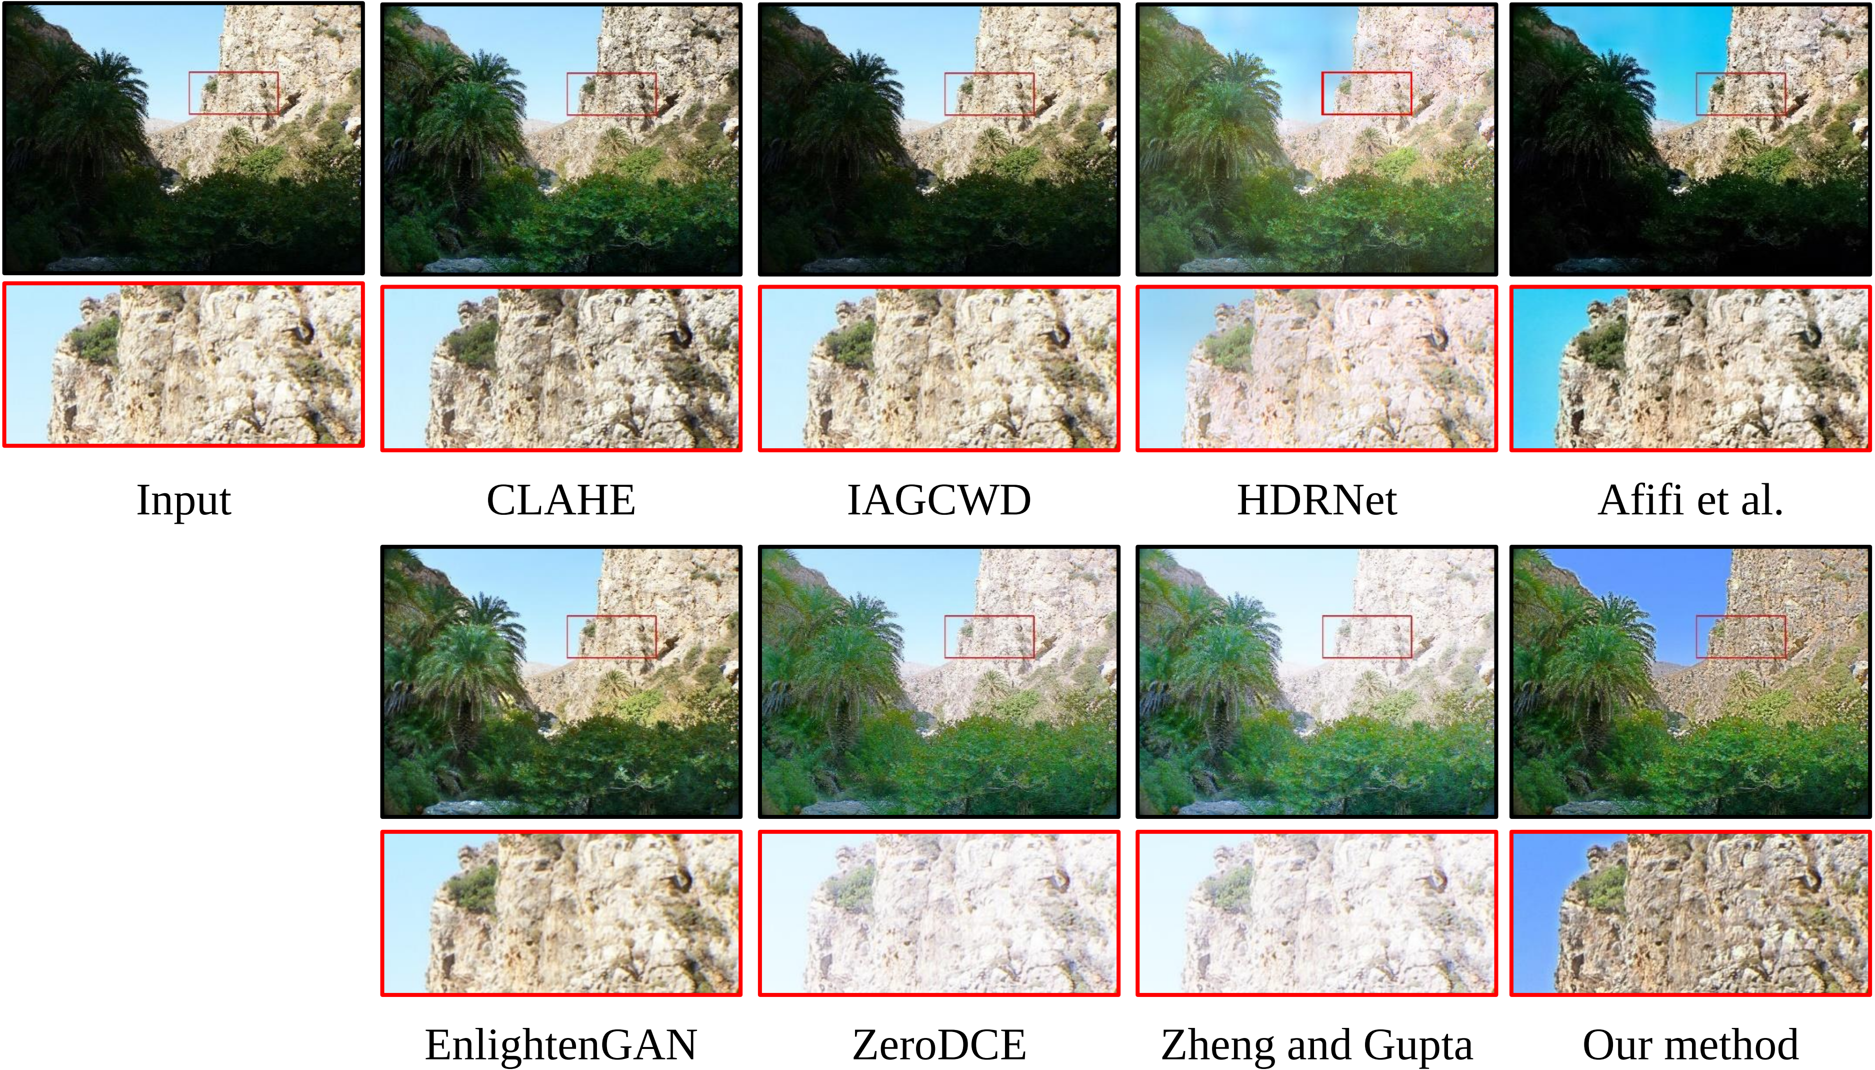
Input
CLAHE
IAGCWD
HDRNet
Afifi et al.
EnlightenGAN
ZeroDCE
Zheng and Gupta
Our method

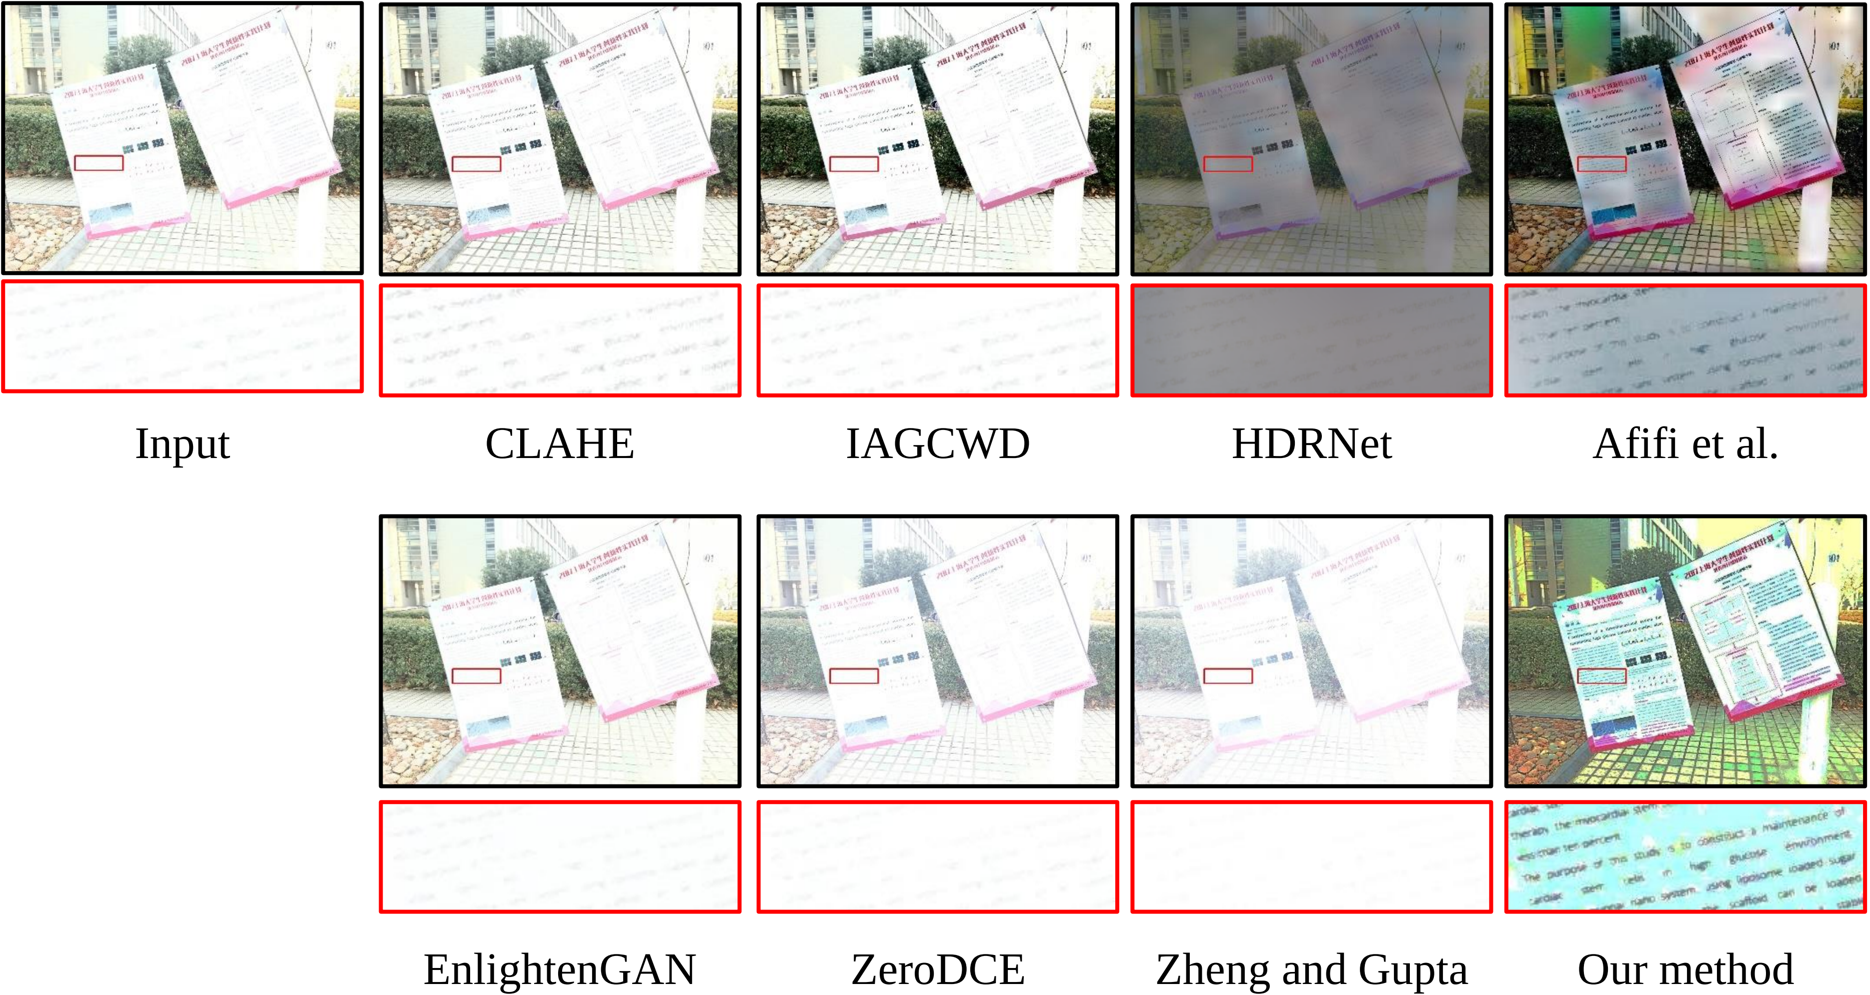
Input
CLAHE
IAGCWD
HDRNet
Afifi et al.
EnlightenGAN
ZeroDCE
Zheng and Gupta
Our method

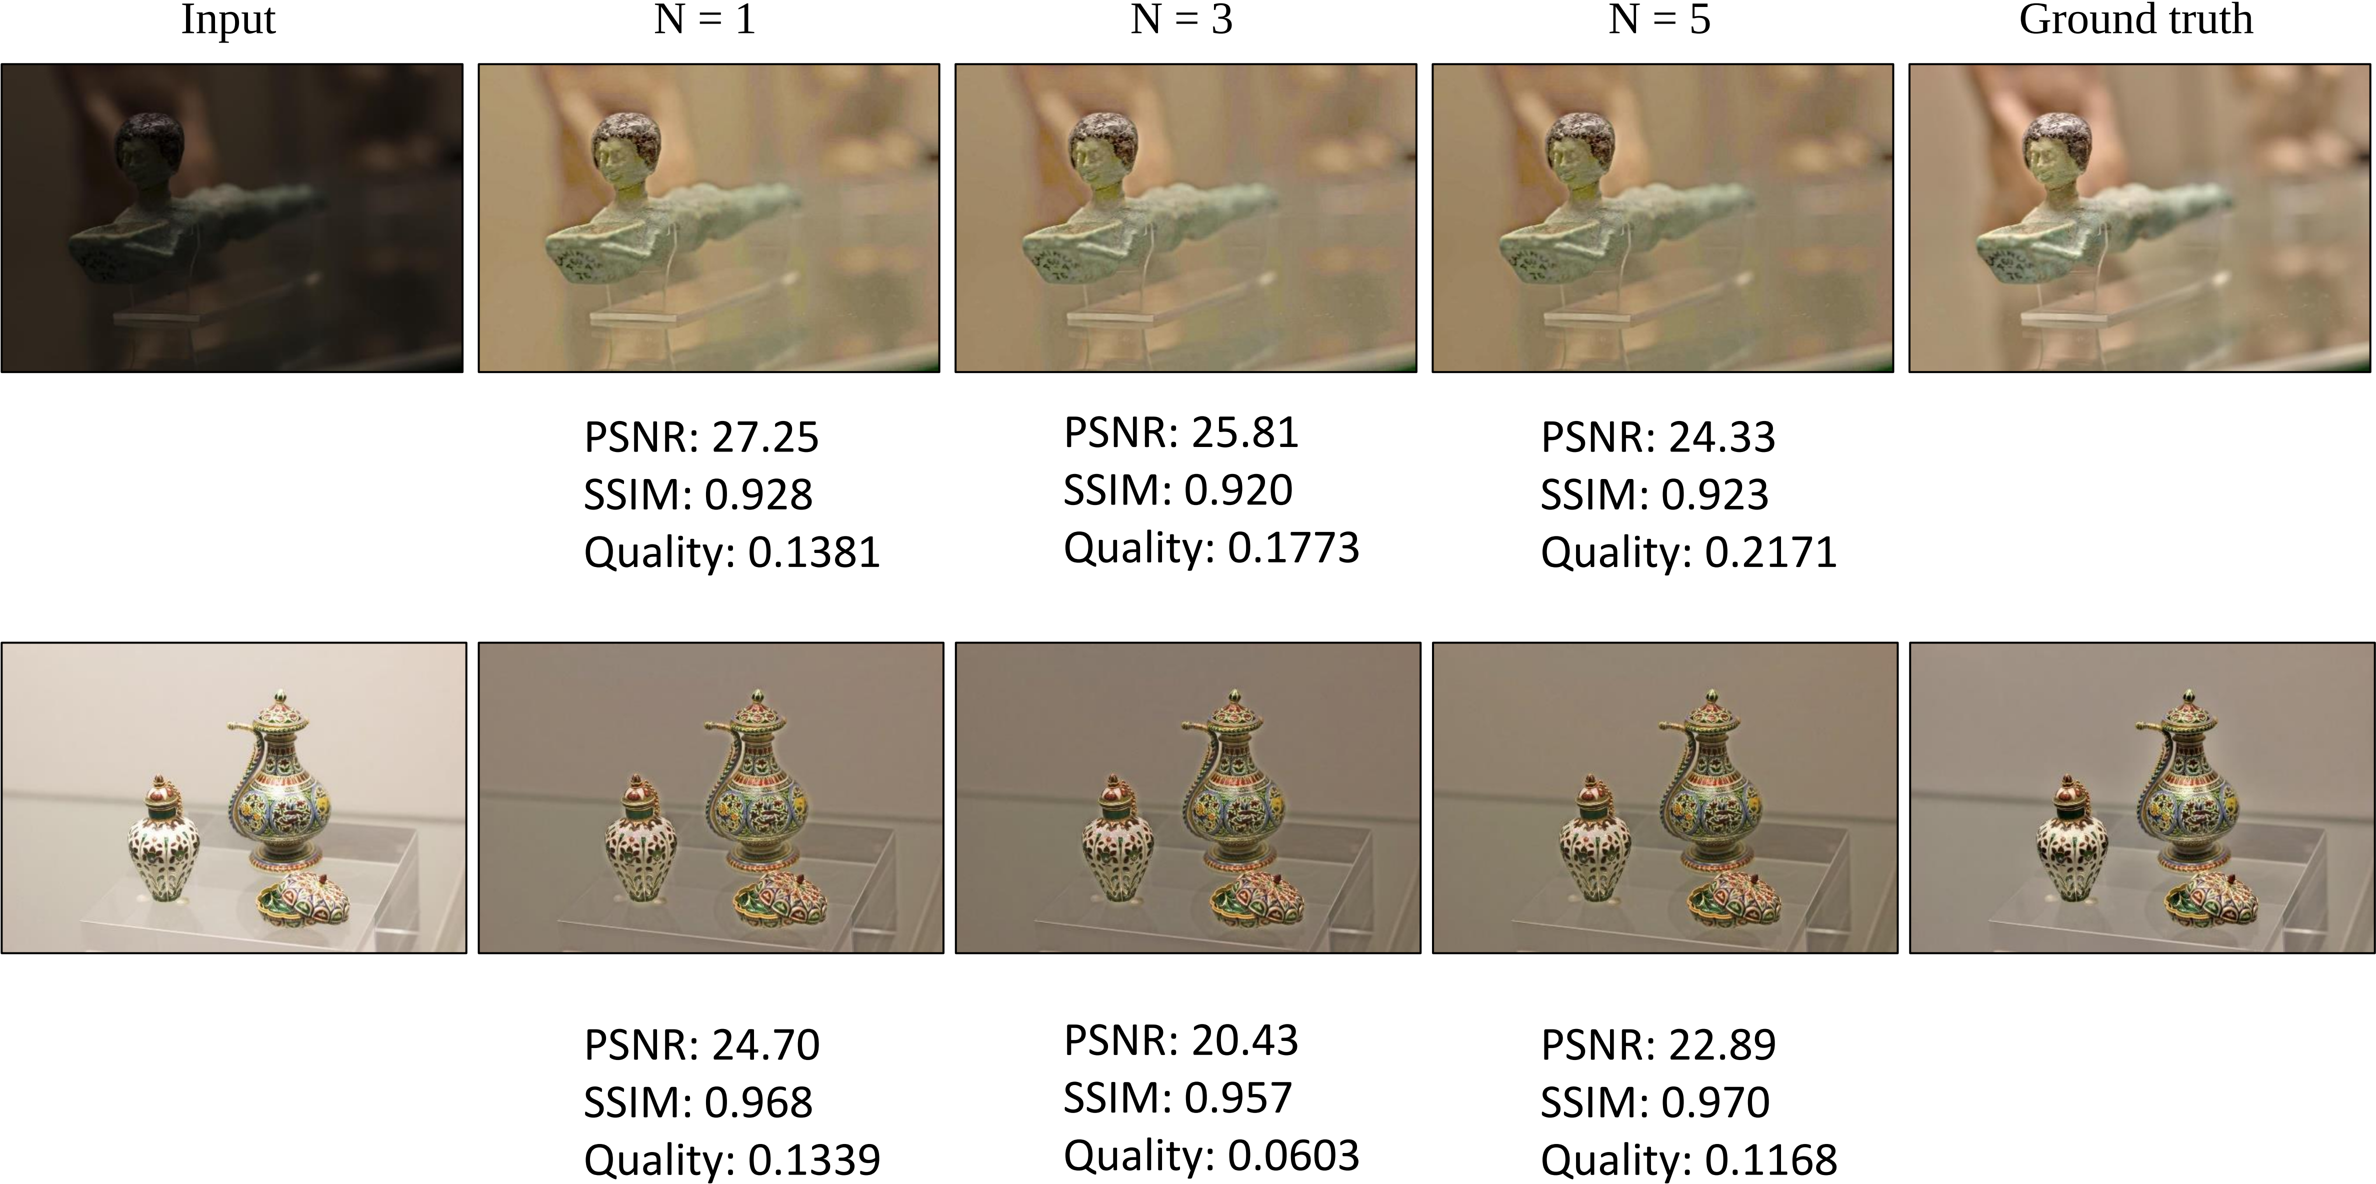
Input
N = 1
N = 3
N = 5
Ground truth
PSNR: 27.25
SSIM: 0.928
Quality: 0.1381
PSNR: 25.81
SSIM: 0.920
Quality: 0.1773
PSNR: 24.33
SSIM: 0.923
Quality: 0.2171
PSNR: 24.70
SSIM: 0.968
Quality: 0.1339
PSNR: 20.43
SSIM: 0.957
Quality: 0.0603
PSNR: 22.89
SSIM: 0.970
Quality: 0.1168

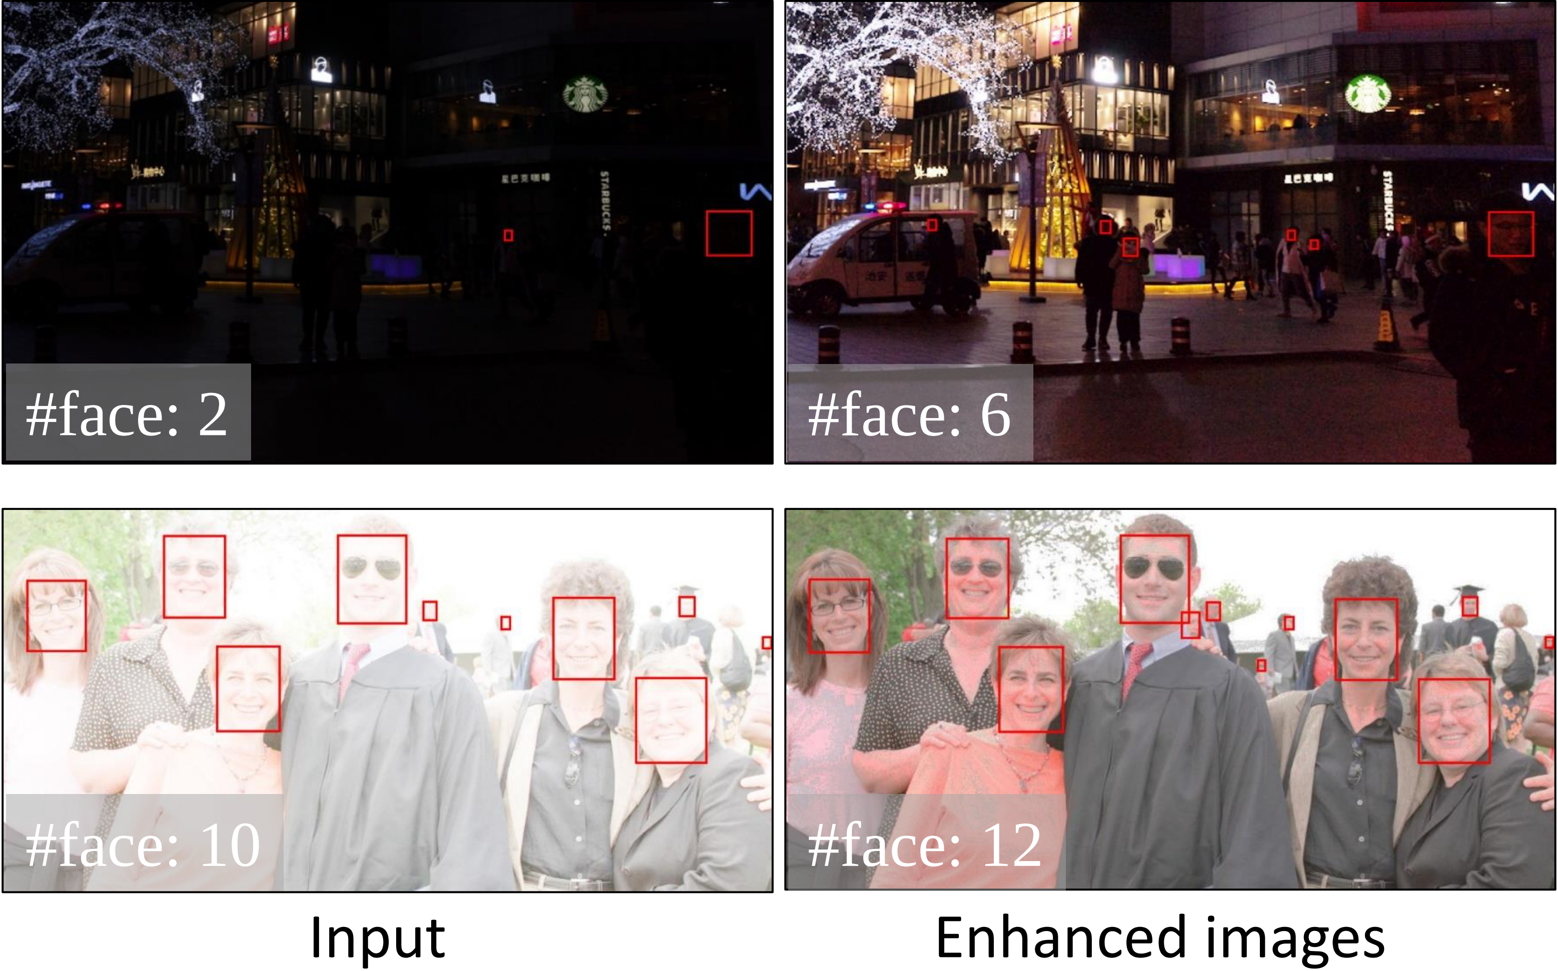
#face: 2
#face: 6
#face: 10
#face: 12
Input
Enhanced images

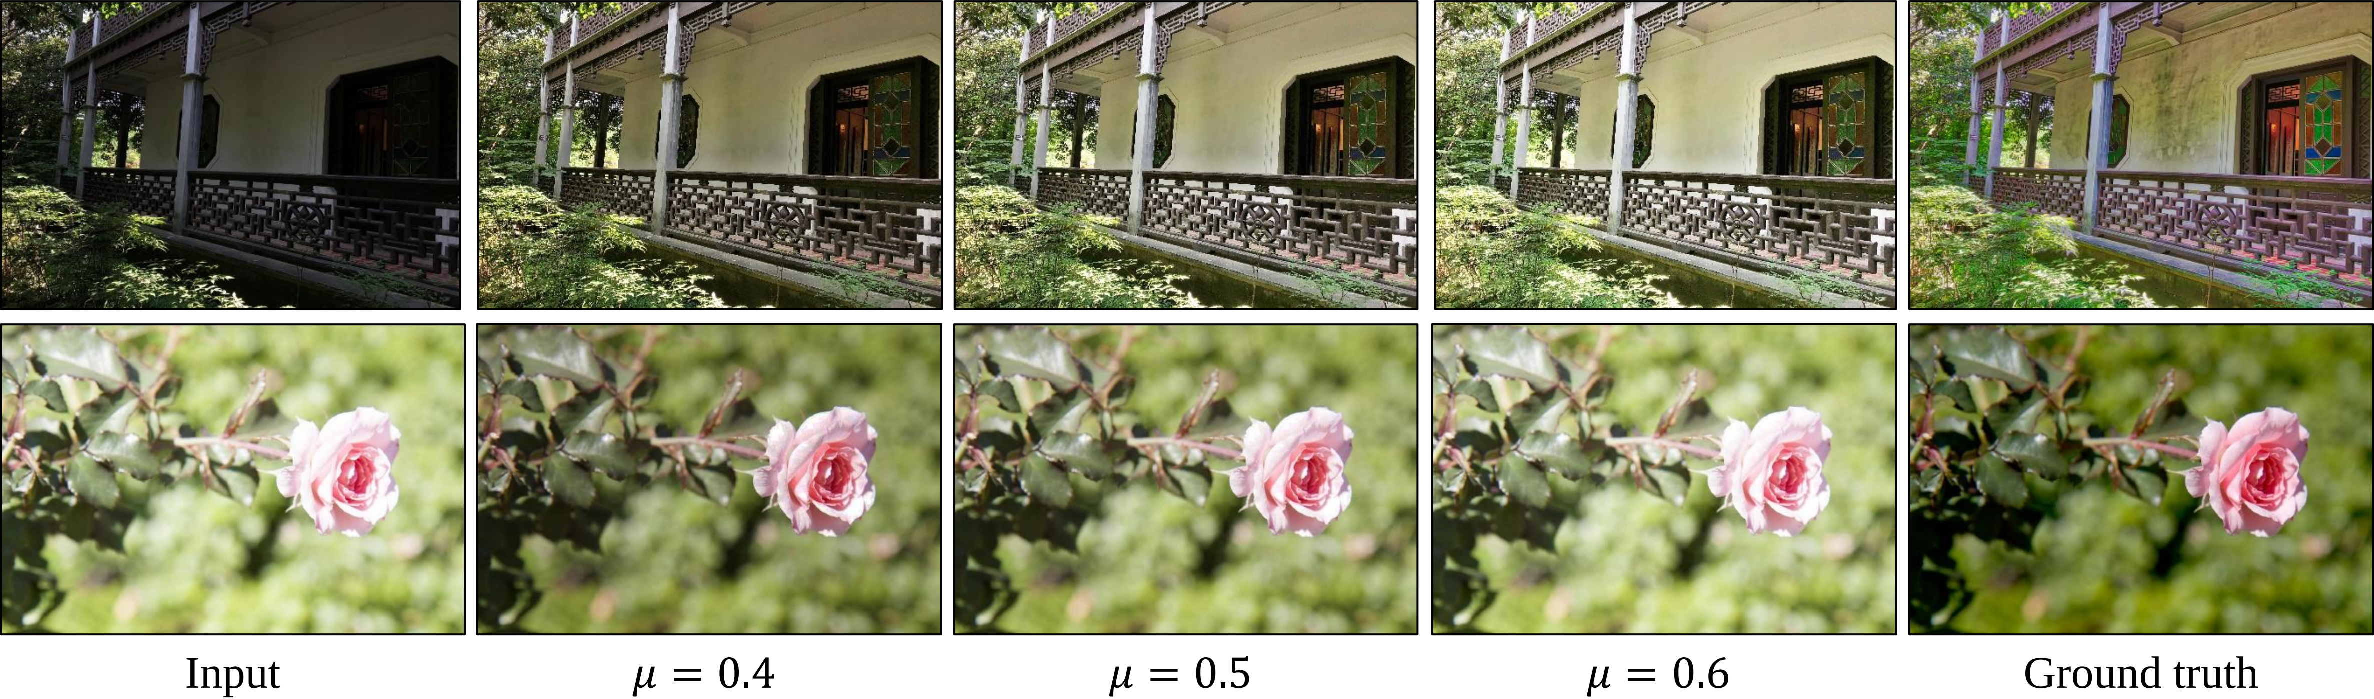
Input
$\mu = 0.4$
$\mu = 0.5$
$\mu = 0.6$
Ground truth

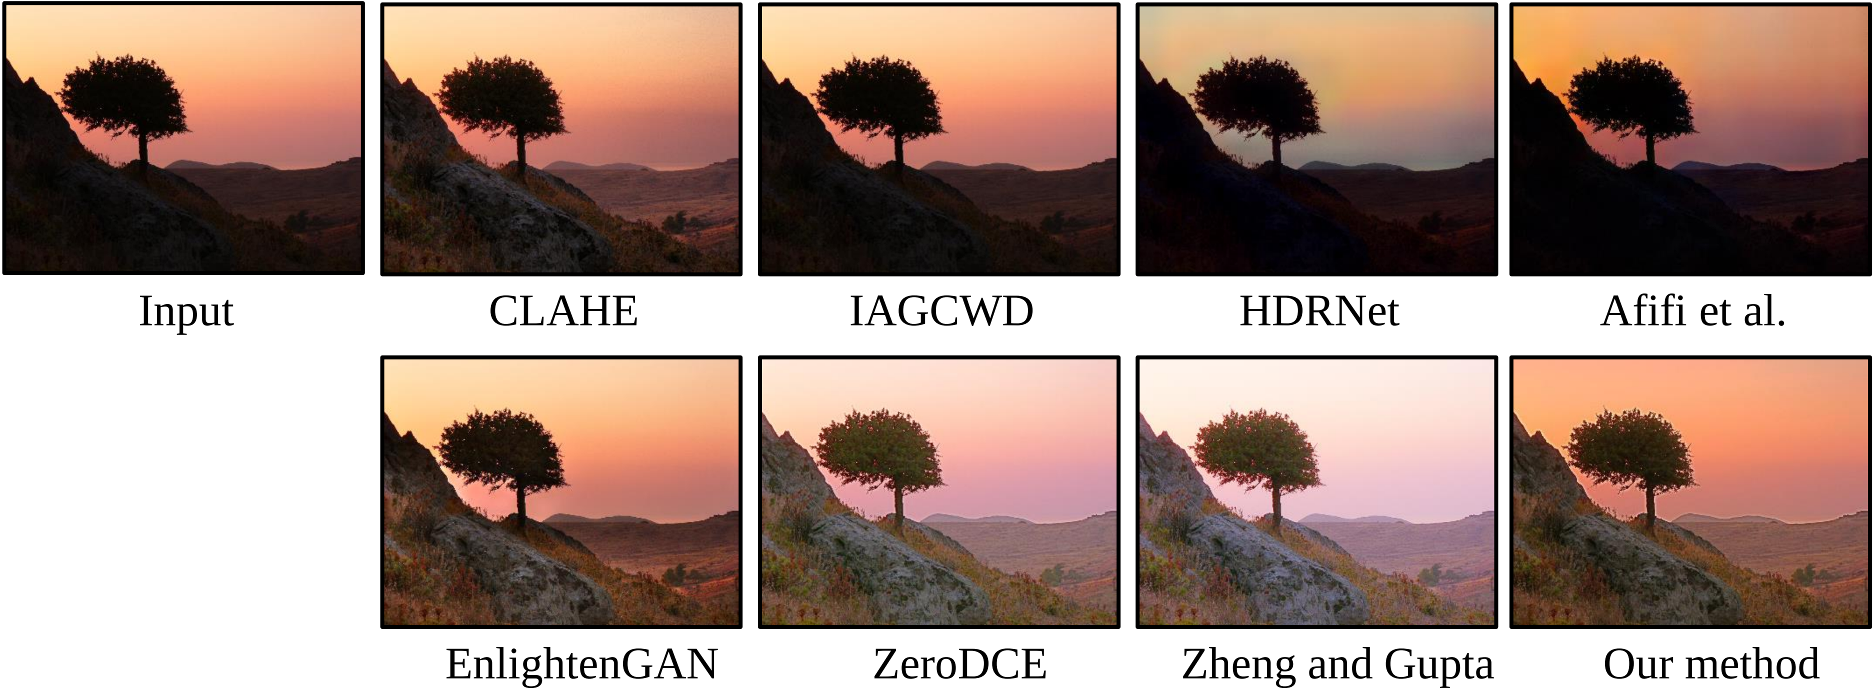
Input
CLAHE
IAGCWD
HDRNet
Afifi et al.
EnlightenGAN
ZeroDCE
Zheng and Gupta
Our method

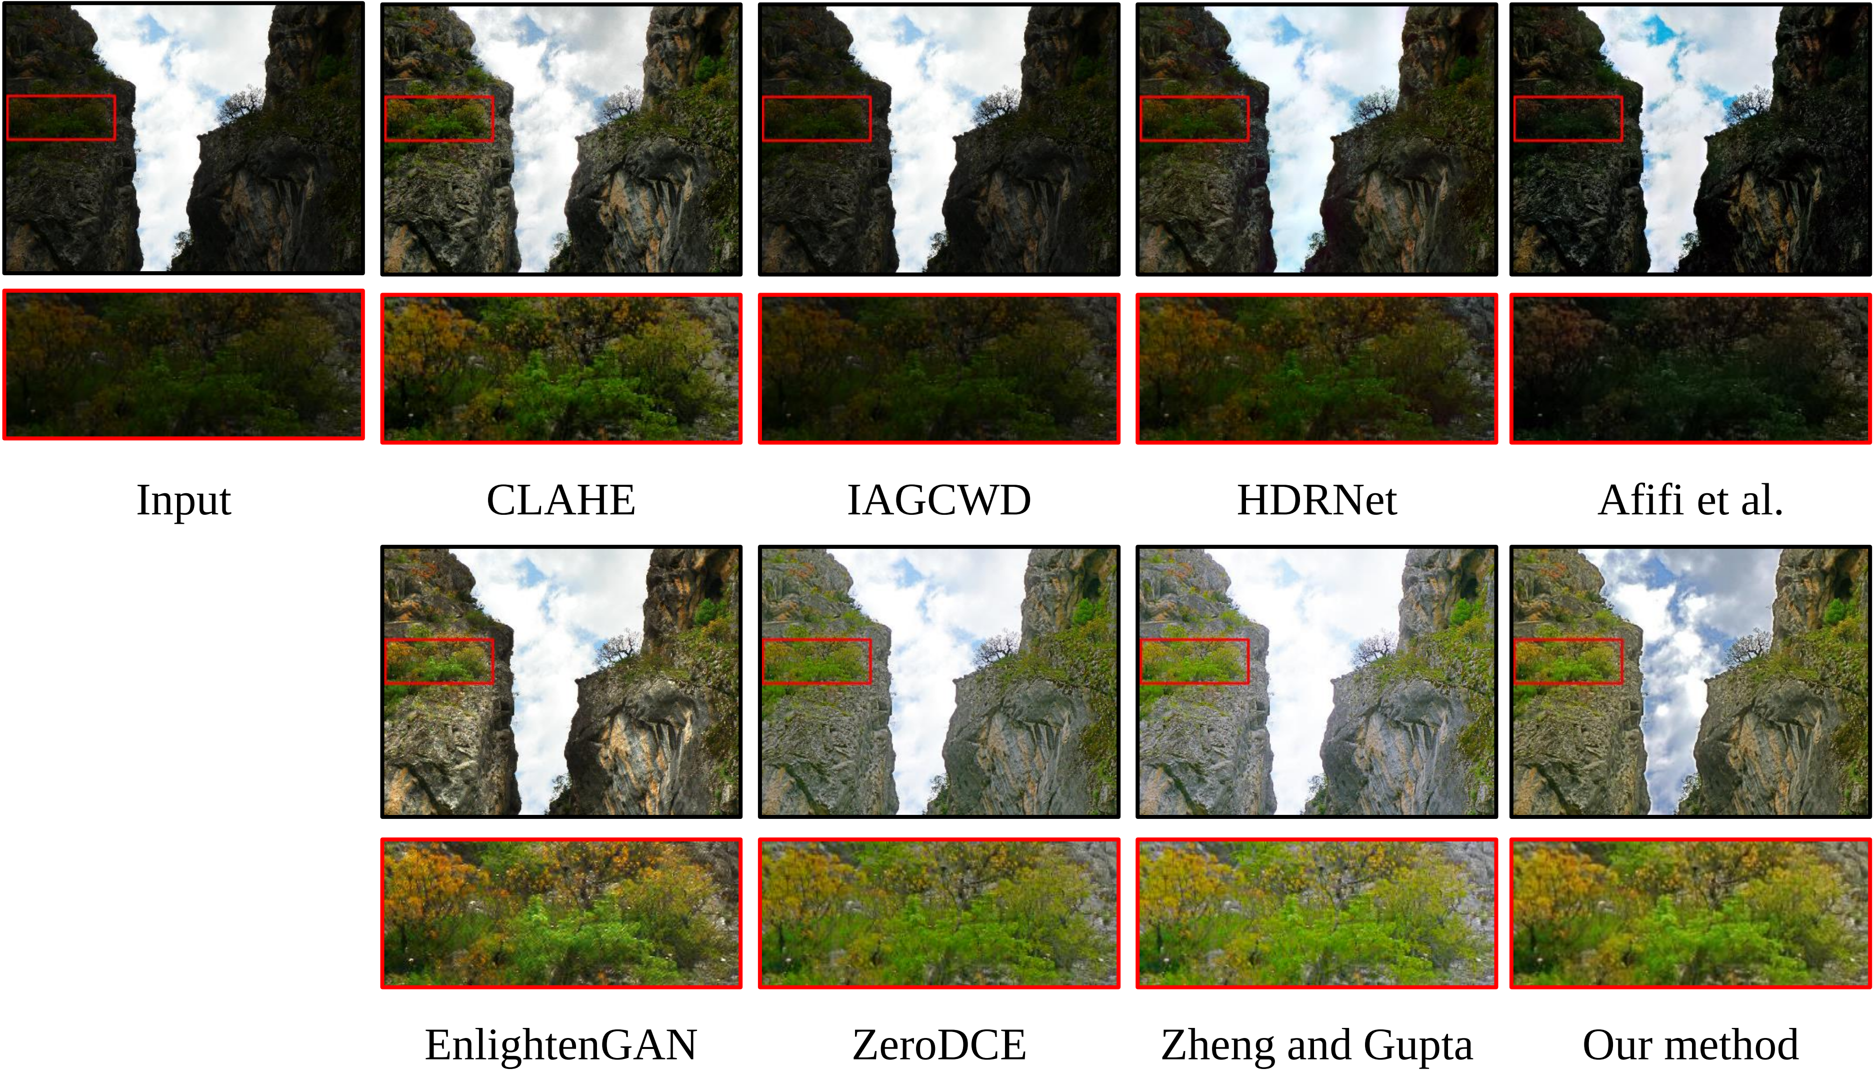
Input
CLAHE
IAGCWD
HDRNet
Afifi et al.
EnlightenGAN
ZeroDCE
Zheng and Gupta
Our method

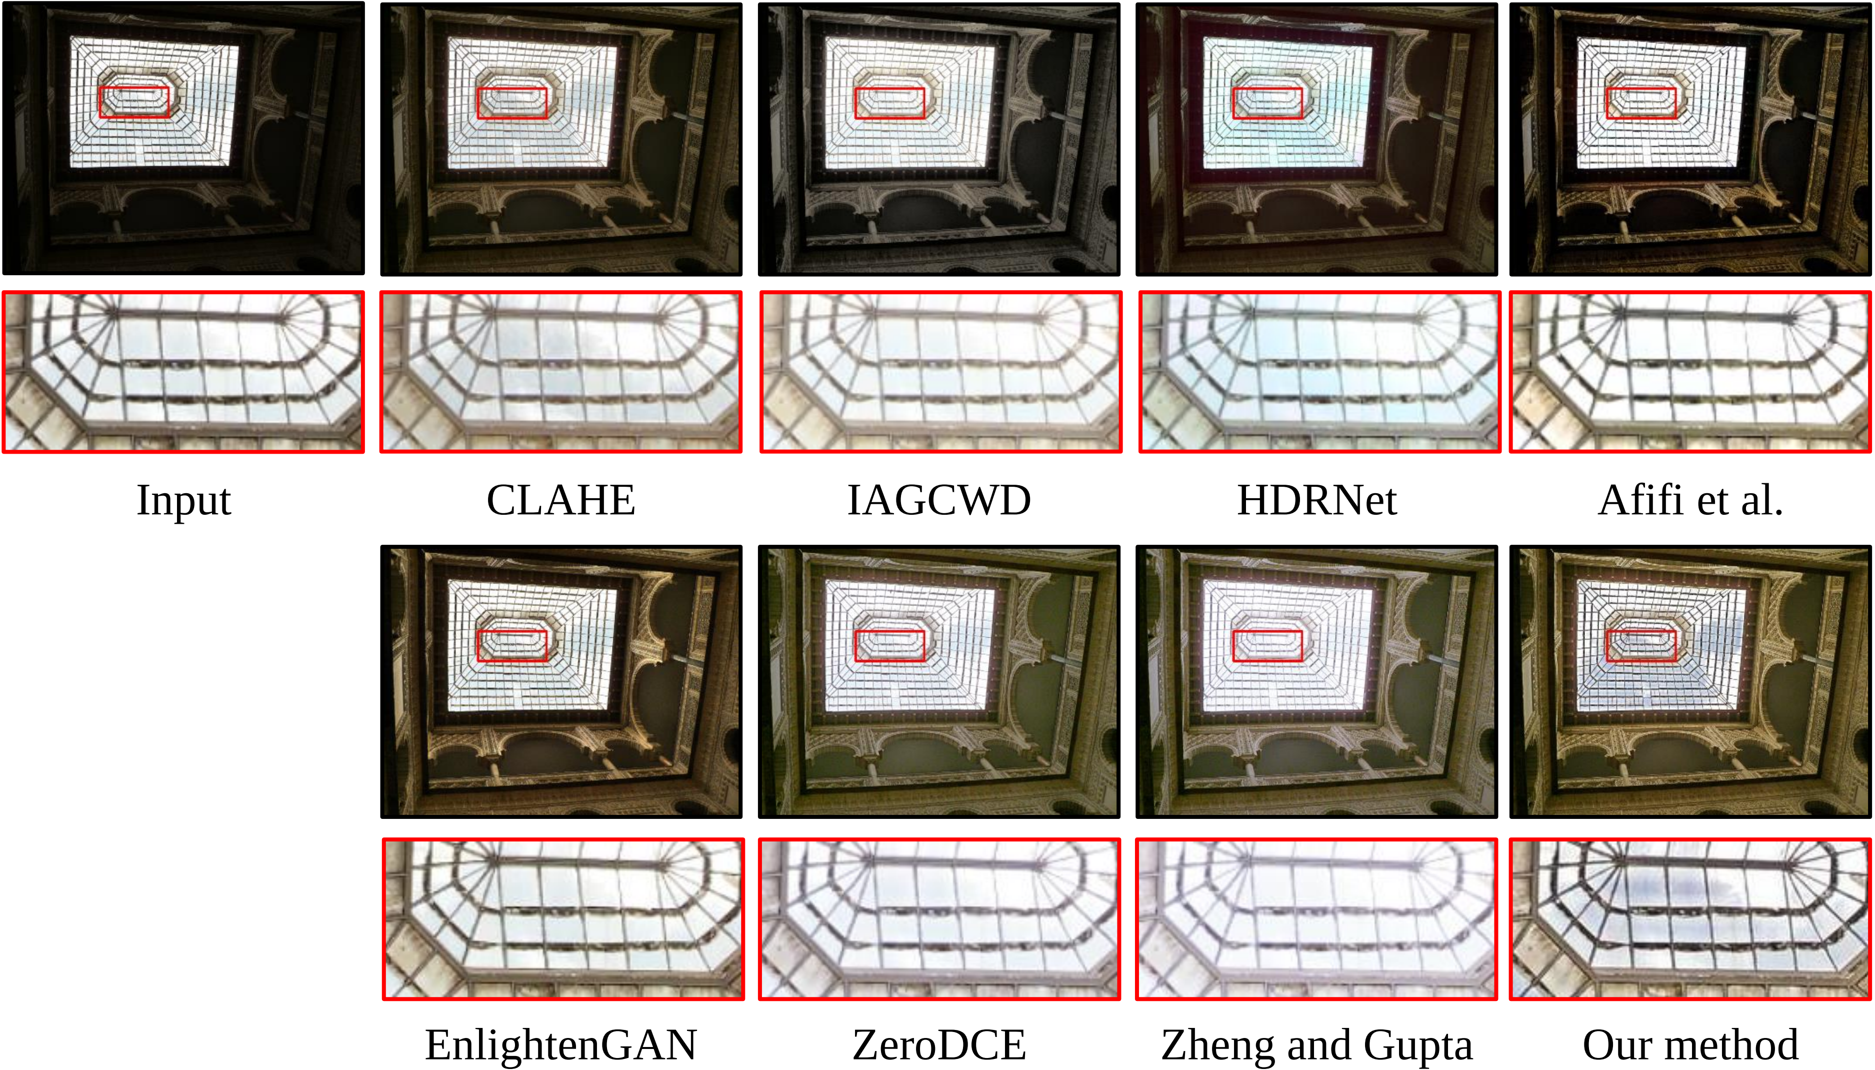
Input
CLAHE
IAGCWD
HDRNet
Afifi et al.
EnlightenGAN
ZeroDCE
Zheng and Gupta
Our method

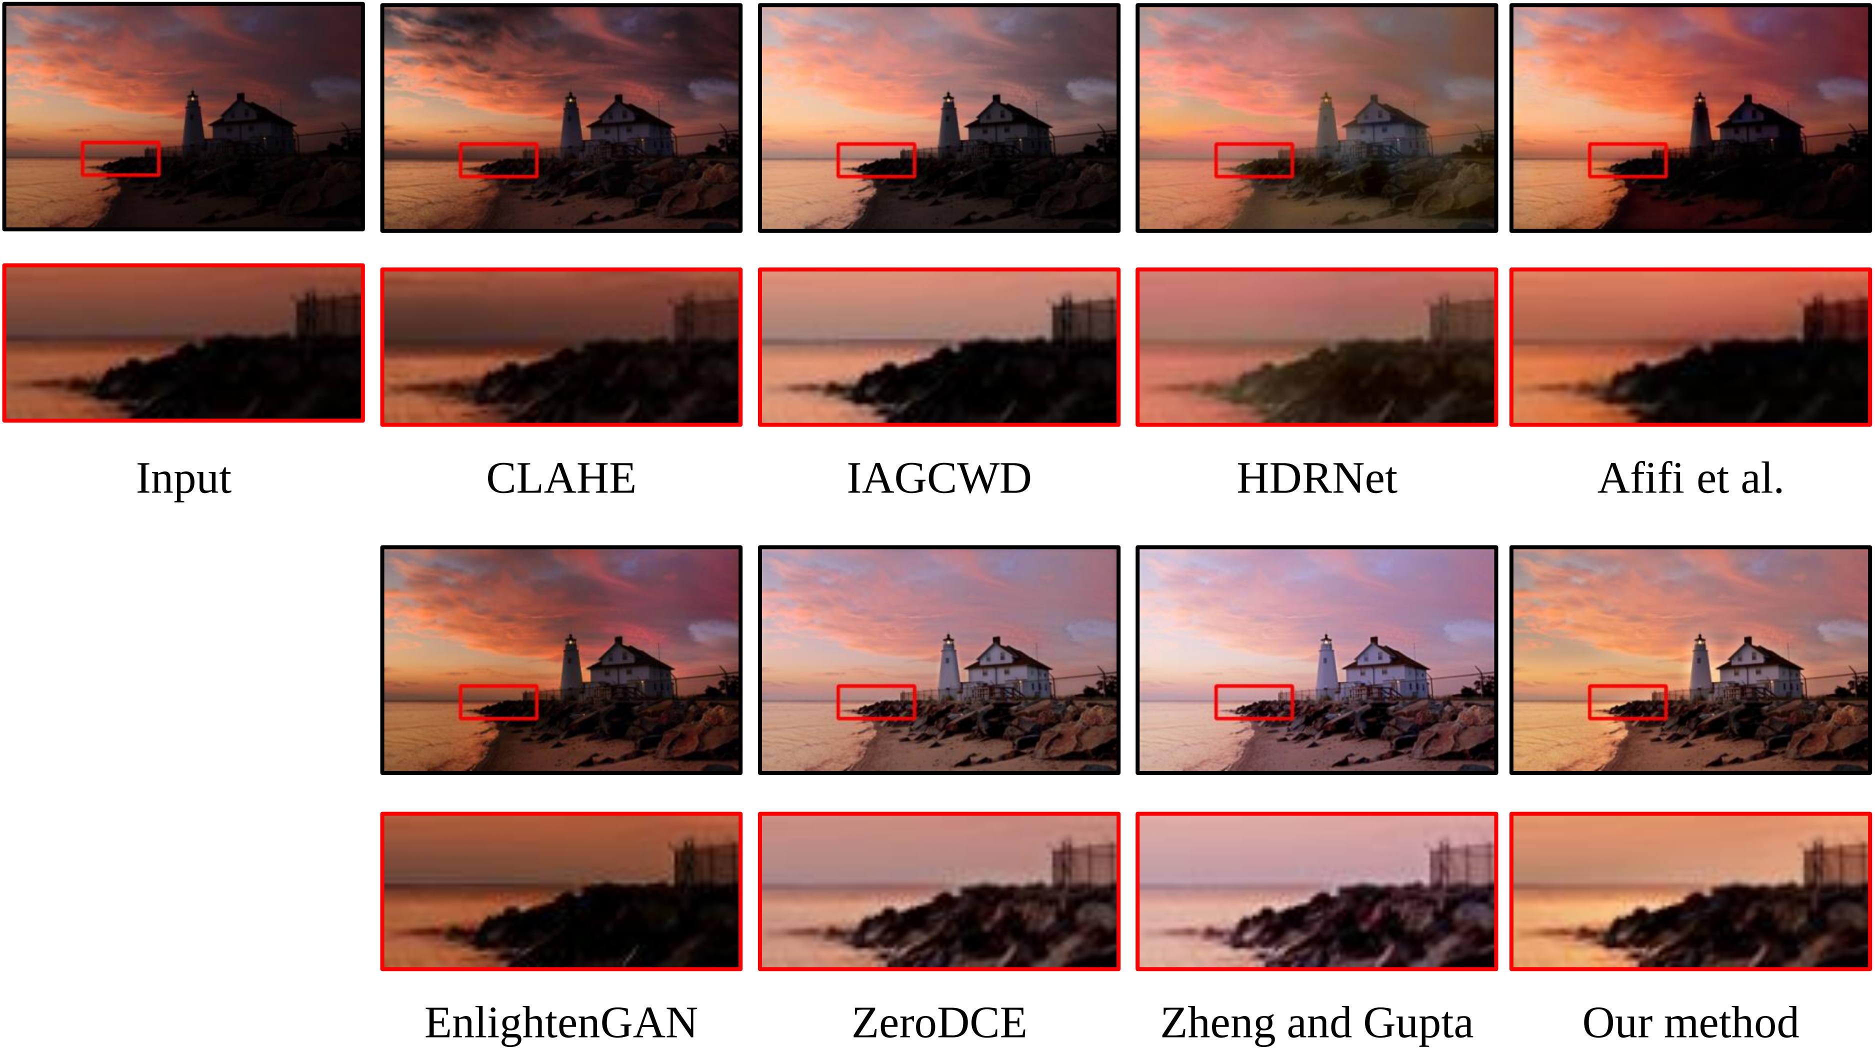
Input
CLAHE
IAGCWD
HDRNet
Afifi et al.
EnlightenGAN
ZeroDCE
Zheng and Gupta
Our method
